# Supplementary material for: Extracting energy from almost unknown quantum states
Source: arXiv:2509.08899 source file (2026-11-26)
Supplement: Supplementary file 1 [file supplemental.tex]

% !TeX document-id = {df27367c-91d5-4350-933d-1dd8175af257}
% !TeX TXS-program:compile = txs:///pdflatex/[--shell-escape]
\documentclass[10pt,aps,prb,supe,nofootinbib,superscriptaddress]{revtex4-2}
\usepackage{xcolor}
\usepackage{float}
\usepackage{dsfont}
\usepackage[utf8]{inputenc}
\usepackage{times,amsmath,amsfonts,amssymb,latexsym,mathtools} 
\usepackage{graphicx}
\usepackage{subfigure}
\usepackage[normalem]{ulem}
\usepackage{physics, outlines, bm}
\usepackage{amsthm}
\usepackage{hyperref}
\hypersetup{colorlinks = true,allcolors = teal}
 %\pmb
\newcommand{\bseq}{\begin{subequations}}
\newcommand{\eseq}{\end{subequations}}

\newtheorem{definition}{Definition}

\usepackage{amsthm}
    \newtheorem{theorem}{Theorem}
    \newtheorem{proposition}[theorem]{Proposition}
    \newtheorem{lemma}[theorem]{Lemma}
    \newtheorem{corollary}{Corollary}[theorem]

\usepackage{mathrsfs}
\renewcommand{\trace}{\operatorname{Tr}}
\usepackage{braket}

\usepackage[]{algorithm2e}

\definecolor{Blues5seq1}{RGB}{239,243,255}
\definecolor{Blues5seq2}{RGB}{189,215,231}
\definecolor{Blues5seq3}{RGB}{107,174,214}
\definecolor{Blues5seq4}{RGB}{49,130,189}
\definecolor{Blues5seq5}{RGB}{8,81,156}

\usepackage{tcolorbox}
\tcbuselibrary{minted,breakable,xparse,skins}

\definecolor{bg}{gray}{0.95}
\DeclareTCBListing{mintedbox}{O{}m!O{}}{%
  breakable=true,
  listing engine=minted,
  listing only,
  minted language=#2,
  minted style=default,
  minted options={%
    linenos,
    gobble=0,
    breaklines=true,
    breakafter=,,
    fontsize=\small,
    numbersep=8pt,
    #1},
  boxsep=0pt,
  left skip=0pt,
  right skip=0pt,
  left=25pt,
  right=0pt,
  top=3pt,
  bottom=3pt,
  arc=5pt,
  leftrule=0pt,
  rightrule=0pt,
  bottomrule=2pt,
  toprule=2pt,
  colback=bg,
  colframe=Blues5seq1,
  enhanced,
  overlay={%
    \begin{tcbclipinterior}
    \fill[Blues5seq5!20!Blues5seq1] (frame.south west) rectangle ([xshift=20pt]frame.north west);
    \end{tcbclipinterior}},
  #3}

\setcounter{page}{1}

\begin{document}
\title{{\Large Supplemental Material}\\Extracting and charging energy into almost unknown quantum states}
\author{Andrea Canzio}
\author{Vasco Cavina}
\author{Roberto Menta}
\author{Vittorio Giovannetti}
\affiliation{NEST, Scuola Normale Superiore, I-56126 Pisa, Italy} 

\maketitle

This Supplemental Material is designed to be read independently from the main text, serving as its extended version. 
Sec.~\ref{sec:min-anti-erg} provides a detailed characterization of the energy-constrained minimum ergotropy and anti-ergotropy with respect to the set of all states with fixed mean energy. 
In this section, we prove the following results presented in the main text: Proposition~1 (Sec.~\ref{subsec:min-anti-passive}), Theorem~2 (Sec.~\ref{subsec:min-state-charac}), and the ergotropy-related results of Theorem~3 (Sec.~\ref{subsec:anti-h-min-erg}). 
Sec.~\ref{sec:algo} presents an illustrative algorithm (implemented in Python) for solving the energy-constrained minimum ergotropy and anti-ergotropy problem. 
Sec.~\ref{sec:implications} derives the upper bounds for coherent ergotropy and anti-ergotropy, as reported in the main text in Eqs.~(16) and~(17). 
The new functionals introduced in this work to quantify the maximum extractable/injectable energy from a quantum state of fixed mean energy in the worst-case scenario, namely max-WCEE and max-WCIE, are analyzed in Sec.~\ref{sec:unknown-ext}. There, we prove additional results stated in the main text: the previously unproven part of Theorem~3 (Sec.~\ref{subsec:anti-h-ext-energy}) and Theorem~4 (Secs.~\ref{subsec:diag} and~\ref{subsec:rand}). 
Furthermore, in Sec.~\ref{subsec:lowerbound}, we derive a lower bound for max-WCEE and max-WCIE that was not included in the main text. 
Explicit calculations for the qutrit example discussed in the main text are reported in Sec.~\ref{sec:qutrit}, where we also present the case $\delta>0$, which was omitted from the main body. 
Finally, we emphasize that all quantities depend explicitly on the Hamiltonian, which we denote here with the superscript $\bullet^{(\hat{H})}$, omitted in the main text for notational simplicity. 
For instance, for the ergotropy we have $\underbrace{\mathcal{E}^{(\hat{H})}(\rho)}_{\text{supplemental}} \longrightarrow \underbrace{\mathcal{E}(\rho)}_{\text{main text}}$.
% \begin{align} \nonumber
%     \overbrace{\mathcal{E}^{(\hat{H})}(\rho)}^{\text{supplemental}}
%     \longrightarrow
%     \overbrace{\mathcal{E}(\rho)}^{\text{main text}} .
% \end{align}

\tableofcontents
\newpage

\section{\label{sec:min-anti-erg}Characterization of the energy-constrained minimum ergotropy/anti-ergotroy}

The aim of this first section is to provide a complete characterization of the minimum values that ergotropy and anti-ergotropy can attain among all states with a fixed mean energy (Eqs.~\eqref{eq:min-erg} and~\eqref{eq:min-anti-erg}), as well as to identify the states that achieve these minima.
We begin by presenting some fundamental properties of ergotropy and anti-ergotropy (Sec.~\ref{subsec:first-prop}), and then proceed to characterize the states that minimize these quantities (Sec.~\ref{subsec:min-diag},~\ref{subsec:min-anti-passive}, and~\ref{subsec:min-state-charac}).
Finally, we examine a special class of Hamiltonians for which the problem simplifies significantly (Sec.~\ref{subsec:anti-h-min-erg}).

\subsection{\label{sec:prob-stat}Problem statement and definitions}

In this introductory section, we will state the main problems that we will tackle and gather most of the definitions.

Let $\Delta E^{(\hat{H})} (\rho,\Lambda)$ be the energy variation between the initial state $\rho$ and the final state $\Lambda(\rho)$ evolved according to the map $\Lambda(\bullet)$, with respect to the Hamiltonian $\hat{H}$:
\begin{align}
    \label{eq:def-delta-e}\Delta E^{(\hat{H})} (\rho,\Lambda)
    \coloneqq
    \trace\! \left[ \rho \hat{H} \right] - \trace\! \left[ \Lambda(\rho) \hat{H} \right] \,.
\end{align}
The maximum extractable energy $\mathcal{E}^{(\hat{H})}(\rho)$ and chargeable energy $\mathcal{A}^{(\hat{H})}(\rho)$ into the state $\rho$ through unitary operations\footnote{Unitary maps are defined as $\mathcal{U}(\bullet) = \hat{U}(\bullet)\hat{U}^\dagger$, where $\hat{U}$ is the unitary operator such that $\hat{U}^\dagger \hat{U} = \mathbb{I}$.} $\mathcal{U}$, called \emph{ergotropy}~\cite{hatsopoulos_unified_1976, A.E.Allahverdyan_2004} and \emph{anti-ergotropy}~\cite{salvia_distribution_2021} respectively, can be written as
\begin{align}
    \label{eq:def-erg}\mathcal{E}^{(\hat{H})}(\rho)
    &\coloneqq \max_{\Lambda \in \mathcal{U}} \left[ \Delta E^{(\hat{H})} (\rho,\Lambda) \right] \,,\\
    \label{eq:def-anti-erg}\mathcal{A}^{(\hat{H})}(\rho)
    &\coloneqq \max_{\Lambda \in \mathcal{U}} \left[ - \Delta E^{(\hat{H})} (\rho,\Lambda) \right] \,.
\end{align}
In Sec.~\ref{sec:min-anti-erg} we will be interested in finding the minimum of these quantities with respect to the set of all the states with mean energy fixed at a given value.
\begin{definition}
     Let $\sigma(\mathcal{H})$ be the space of quantum states defined on the Hilbert space $\mathcal{H}$, we call $\sigma_E^{(\hat{H})} \subset \sigma(\mathcal{H})$ the space of all states at energy $E$ with respect to the Hamiltonian $\hat{H}$,
    \begin{align}
        \sigma_E^{(\hat{H})}
        \coloneqq
        \left\{ \rho\in\sigma(\mathcal{H}) \mid \trace\! \left[ \rho \hat{H} \right] = E \right\} \,.
\end{align}
\end{definition}
Note that, being $\sigma(\mathcal{H})$ a convex and compact space, any subset obtained through a linear constraint -- such as $\sigma_E^{(\hat{H})}$ -- will also be convex and compact.

\begin{definition}
    We call $\mathcal{E}_{\text{min}}^{(\hat{H})}(E)$ and $\mathcal{A}_{\text{min}}^{(\hat{H})}(E)$ the minimum value of the ergotropy and anti-ergotropy with respect to all the states having mean energy $E$, i.e.,
    \begin{align}
        \label{eq:min-erg}
        \mathcal{E}_{\text{min}}^{(\hat{H})}(E)
        &\coloneqq \min_{\rho\in\sigma_E^{(\hat{H})}} \mathcal{E}^{(\hat{H})}(\rho) \,,\\
        \label{eq:min-anti-erg}
        \mathcal{A}_{\text{min}}^{(\hat{H})}(E)
        &\coloneqq \min_{\rho\in\sigma_E^{(\hat{H})}} \mathcal{A}^{(\hat{H})}(\rho) \,.
    \end{align}
\end{definition}

To characterize the energy-constrained minimum ergotropy (anti-ergotropy) and the states which achieve it, we will make use of many subspaces of $\sigma_E^{(\hat{H})}$. 
An important subspace of it is the one of states which commute with the Hamiltonian of the system.
\begin{definition}
    We call $\Delta_E^{(\hat{H})}$ the set of all states having mean energy $E$ and commuting with the Hamiltonian $\hat{H}$,
    \begin{align}
        \Delta_E^{(\hat{H})}
        \coloneqq \left\{ \rho\in\sigma_E^{(\hat{H})} \mid \left[\rho,\hat{H}\right] = 0 \right\} \,.
    \end{align}
\end{definition}
Furthermore, we will be interested in the states which have an ordered spectrum and the characterization of the spaces of such states.
\begin{definition}\label{def:anti-pass}
    A state is called passive (anti-passive) and labelled as $\rho^\downarrow$ ($\rho^\uparrow$) with respect to the Hamiltonian $\hat{H}$, when it is diagonal with respect to $\hat{H}$, $\rho^\downarrow \in \Delta_E^{(\hat{H})}$ ($\rho^\uparrow \in \Delta_E^{(\hat{H})}$) and its eigenvalues are in decreasing (increasing) order with respect to the ordered Hamiltonian basis\footnote{When the Hamiltonian spectrum is degenerate, we assume we can always choose the basis in the degenerate subspace as we prefer.} $\{\ket{\epsilon_i}\}$, i.e.,
    \begin{align}
        \rho^\downarrow
        &= \sum_i \lambda_i^\downarrow \ket{\epsilon_i} \bra{\epsilon_i} \,,\\
        \rho^\uparrow
        &= \sum_i \lambda_i^\uparrow \ket{\epsilon_i} \bra{\epsilon_i} \,,
    \end{align}
    where $\epsilon_{i+1}\geq\epsilon_i$, $\lambda_{i+1}^\downarrow \leq \lambda_i^\downarrow$, and $\lambda_{i+1}^\uparrow \geq \lambda_i^\uparrow$.
    We label $\Delta_{E,\downarrow}^{(\hat{H})}$ ($\Delta_{E,\uparrow}^{(\hat{H})}$)  the subspace of $\Delta_E^{(\hat{H})}$ that contains only the passive (anti-passive) states.
\end{definition}
\begin{definition}\label{def:anti-pass-spaces}
    The spaces of all passive and anti-passive states with respect to the Hamiltonian $\hat{H}$ are called $\Delta_{\downarrow}^{(\hat{H})}$ and $\Delta_{\uparrow}^{(\hat{H})}$ respectively, i.e.,
    \begin{align}
        \label{eq:def-passive-set}
        \Delta_{\downarrow}^{(\hat{H})}
        &\coloneqq \left\{ \rho^\downarrow \in \sigma(\mathcal{H}) \mid \rho^\downarrow = \sum_{k} \lambda_k^\downarrow \ket{\epsilon_k} \bra{\epsilon_k} \,,\, \lambda_{k+1}^\downarrow \leq \lambda_k^\downarrow \right\} \,,\\
        \label{eq:def-anti-passive-set}
        \Delta_{\uparrow}^{(\hat{H})}
        &\coloneqq \left\{ \rho^\uparrow \in \sigma(\mathcal{H}) \mid \rho^\uparrow = \sum_{k} \lambda_k^\uparrow \ket{\epsilon_k} \bra{\epsilon_k} \,,\, \lambda_{k+1}^\uparrow \geq \lambda_k^\uparrow \right\} \, .
    \end{align}
\end{definition}
Note that, by construction, we have $\Delta_{E, \downarrow}^{(\hat{H})} = \sigma_E^{(\hat{H})} \cap \Delta_{\downarrow}^{(\hat{H})}$ and $\Delta_{E, \uparrow}^{(\hat{H})} = \sigma_E^{(\hat{H})} \cap \Delta_{\uparrow}^{(\hat{H})}$.

\subsection{\label{subsec:first-prop}First properties of the energy-constrained minimum ergotropy/anti-ergotropy}

We start by showing some properties of the ergotropy and anti-ergotropy that we will use in what follows.
First, we show that these functionals are convex with respect to input states.
\begin{proposition}\label{prop:convErg}
    The ergotropy functional $\mathcal{E}^{(\hat{H})}(\rho)$ and the anti-ergotropy functional $\mathcal{A}^{(\hat{H})}(\rho)$ are convex with respect to the input state $\rho$, i.e., $\forall \rho_1, \rho_2 \in \sigma(\mathcal{H}), \forall p \in [0,1]$,
    \begin{align}
        \mathcal{E}^{(\hat{H})} \left(p\rho_1 + (1-p)\rho_2 \right)
        &\leq p \mathcal{E}^{(\hat{H})}(\rho_1) + (1-p) \mathcal{E}^{(\hat{H})}(\rho_2) \,,\\
        \mathcal{A}^{(\hat{H})}\left(p\rho_1 + (1-p)\rho_2\right)
        &\leq p \mathcal{A}^{(\hat{H})}(\rho_1) + (1-p) \mathcal{A}^{(\hat{H})}(\rho_2) \,.
    \end{align}
\end{proposition}
\begin{proof}
    Let $\Bar{\rho} = p\rho_1 + (1-p)\rho_2$ be a convex sum of $\rho_1$ and $\rho_2$, then
    \begin{align}
        \mathcal{E}^{(\hat{H})}(\Bar{\rho})
        &= p \trace\! \left[ \rho_1 \hat{H} \right] + (1-p) \trace\! \left[ \rho_2 \hat{H} \right] - \min_{\Lambda \in \mathcal{U}} \left( p \trace\! \left[ \Lambda(\rho_1) \hat{H} \right] + (1-p)\trace\! \left[ \Lambda(\rho_2) \hat{H} \right] \right) \;,\\
        &\leq p \trace\! \left[ \rho_1 \hat{H} \right] + (1-p) \trace\! \left[ \rho_2 \hat{H} \right] - \left( p \min_{\Lambda \in \mathcal{U}} \trace\! \left[ \Lambda(\rho_1) \hat{H} \right] + (1-p) \min_{\Lambda \in \mathcal{U}} \trace\! \left[ \Lambda(\rho_2) \hat{H} \right] \right) \;,\\
        &= p \left( \trace\! \left[ \rho_1 \hat{H} \right] - \min_{\Lambda \in \mathcal{U}} \trace\! \left[ \Lambda(\rho_1) \hat{H} \right] \right) + (1-p) \left( \trace\! \left[ \rho_2 \hat{H} \right] - \min_{\Lambda \in \mathcal{U}} \trace\! \left[ \Lambda(\rho_2) \hat{H} \right] \right) \,,\\
        &= p \mathcal{E}^{(\hat{H})}(\rho_1) + (1-p) \mathcal{E}^{(\hat{H})}(\rho_2) \;,
    \end{align}
    where we used the linearity of the trace and the superadditivity of the minimum function.
    The same steps can be repeated for the anti-ergotropy (for which we will exploit the subadditivity of the maximum function), which completes the proof.
\end{proof}
From this result, it follows that the energy-constrained minimum ergotropy and anti-ergotropy are also convex with respect to their argument, the mean energy:
\begin{corollary}\label{cor:convMinErg}
    The energy-constrained minimum ergotropy $\mathcal{E}_{\text{min}}^{(\hat{H})}(E)$ and energy-constrained minimum anti-ergotropy $\mathcal{A}_{\text{min}}^{(\hat{H})}(E)$ are convex functions with respect to the mean energy $E$.
\end{corollary}
\begin{proof}
    Let $\rho_1$ and $\rho_2$ be the states of minimum ergotropy with respect to the mean energy $E_1$ and $E_2$, i.e.,
    \begin{align}
        \rho_1 &= \arg \min_{\rho\in\sigma_{E_1}^{(\hat{H})}} \mathcal{E}^{(\hat{H})}(\rho) \,,\\
        \rho_2 &= \arg \min_{\rho\in\sigma_{E_2}^{(\hat{H})}} \mathcal{E}^{(\hat{H})}(\rho) \,.
    \end{align}
    Let us assume without loss of generality that $E_1 \leq E_2$.
    Then we can define the state $\Bar{\rho} = p \rho_1 + (1-p) \rho_2$ which, varying $p$, has energy $E = p E_1 + (1-p) E_2$.
    By construction, exploiting the convexity of the ergotropy, we will have:
    \begin{align}
        \mathcal{E}_{\text{min}}^{(\hat{H})}(p E_1 + (1-p)E_2)
        &\leq \mathcal{E}^{(\hat{H})}(\Bar{\rho}) \,,\\
        &= \mathcal{E}^{(\hat{H})}(p \rho_1 + (1-p) \rho_2) \,,\\
        &\leq p \mathcal{E}^{(\hat{H})}(\rho_1) + (1-p) \mathcal{E}^{(\hat{H})}(\rho_2) \,,\\
        &= p \mathcal{E}_{\text{min}}^{(\hat{H})}(E_1) + (1-p) \mathcal{E}_{\text{min}}^{(\hat{H})}(E_2) \,.
    \end{align}
    By repeating the exact same steps for the anti-ergotropy, we complete the proof.
\end{proof}

We are now ready to start the characterization of the states of energy-constrained minimum ergotropy and anti-ergotropy.

\subsection{\label{subsec:min-diag}The energy constrained minimum ergotropy/anti-ergotropy is always achieved by a diagonal state}

We first want to show that the minimum value of ergotropy and anti-ergotropy with respect to the states at fixed mean energy is always achieved by states that commute with the Hamiltonian.
The following lemma will be crucial to prove in the next section the equivalent of Prop.~1 of the main text.
\begin{lemma}
\label{lemma2}\label{lemma:minAreDiagonal}
    The energy-constrained minimum ergotropy and anti-ergotropy at fixed mean energy are always achieved by a state that commutes with the Hamiltonian, i.e.,
    \begin{align}
        \mathcal{E}_{\text{min}}^{(\hat{H})}(E)
        &= \min_{\rho\in \Delta_E^{(\hat{H})}} \mathcal{E}^{(\hat{H})}(\rho) \,,\\
        \mathcal{A}_{\text{min}}^{(\hat{H})}(E)
        &= \min_{\rho\in \Delta_E^{(\hat{H})}} \mathcal{A}^{(\hat{H})}(\rho) \,.
    \end{align}
\end{lemma}
\begin{proof}
We will prove this result by showing that from every $\rho\in\sigma_E^{(\hat{H})}$ we can construct another $\Tilde{\rho}\in \Delta_E^{(\hat{H})}$ such that $\mathcal{E}^{(\hat{H})}(\Tilde{\rho}) \leq \mathcal{E}^{(\hat{H})}(\rho)$.
Let $\rho = \sum_{i=1}^d \lambda_i \ket{\phi_i} \bra{\phi_i} \in \sigma_E^{(\hat{H})}$ be a generic state with mean energy $E$ written in its spectral decomposition.
Its ergotropy and anti-ergotropy can be written as
\begin{align}
    \mathcal{E}^{(\hat{H})}(\rho)
    &= \max_{\Lambda \in \mathcal{U}} \left[ \Delta E^{(\hat{H})} (\rho,\Lambda) \right] \,,\\
    &= E - \min_{\Lambda \in \mathcal{U}} \trace\! \left[ \Lambda(\rho) \hat{H} \right] \,,\\
    &= E - \boldsymbol{\lambda}^\downarrow \cdot \boldsymbol{\epsilon}^\uparrow \,,\\
    \mathcal{A}^{(\hat{H})}(\rho)
    &= \max_{\Lambda \in \mathcal{U}} \left[ - \Delta E^{(\hat{H})} (\rho,\Lambda) \right] \,,\\
    &= \max_{\Lambda \in \mathcal{U}} \trace\! \left[ \Lambda(\rho) \hat{H} \right] - E \,,\\
    &= \boldsymbol{\lambda}^\uparrow \cdot \boldsymbol{\epsilon}^\uparrow - E \,,\\
\end{align}
where $\boldsymbol{\lambda}^\downarrow$ ($\boldsymbol{\lambda}^\uparrow$) is the vector of the eigenvalues of $\rho$ in decreasing order: $(\boldsymbol{\lambda}^\downarrow)_{i+1} \leq (\boldsymbol{\lambda}^\downarrow)_i$ (increasing order $(\boldsymbol{\lambda}^\uparrow)_{i+1} \geq (\boldsymbol{\lambda}^\uparrow)_i$); $\boldsymbol{\epsilon}^\uparrow$ is the vector of the eigenvalues of $\hat{H} = \sum_{i=1}^d \epsilon_i \ket{\epsilon_i} \bra{\epsilon_i}$ in increasing order, and the dot represents the standard scalar product between real vectors~\cite{salvia_distribution_2021}.

Now consider the energy-preserving quantum channel $\Omega$ that kills the coherences with respect to the Hamiltonian eigenvector basis \footnote{Note that this quantum channel is not uniquely defined if the energies are degenerate; any choice is good for the purposes of our proof.}:
\begin{align}
    \Tilde{\rho} = \Omega(\rho)
    &\coloneqq \sum_{i=1}^d \braket{\epsilon_i|\rho|\epsilon_i} \ket{\epsilon_i} \bra{\epsilon_i} \,,\\
    &= \sum_{i,j=1}^d \lambda_j |\braket{\phi_j|\epsilon_i}|^2 \ket{\epsilon_i} \bra{\epsilon_i} \,,\\
    &= \sum_{i=1}^d (M \boldsymbol{\lambda})_i \ket{\epsilon_i} \bra{\epsilon_i} \,, \label{eq:diagrho}
\end{align}
where $M_{ij} \coloneqq |\braket{\phi_j|\epsilon_i}|^2$.
Note that $\Tilde{\rho}\in \Delta_E^{(\hat{H})}$, i.e., is diagonal and has the same energy by construction.
The matrix $M$ is a doubly stochastic matrix; thus, we can write it as a convex sum of permutations $M = \sum_{\pi\in\mathcal{S}_d} p_\pi \pi$, where $\sum_\pi p_\pi = 1$ and $\pi\in\mathcal{S}_d$ are $d$-dimensional permutation matrices~\cite{DUFOSSE2016108}.
It follows that the state $\Tilde{\rho}$ can be written as
\begin{align}
    \Tilde{\rho}
    &= \sum_{i=1}^d \left[ \sum_{\pi\in\mathcal{S}_d} p_\pi \left(\pi \boldsymbol{\lambda} \right) \right]_i \ket{\epsilon_i} \bra{\epsilon_i} \,,\\
    &\equiv \sum_{i=1}^d (\boldsymbol{\gamma})_i \ket{\epsilon_i} \bra{\epsilon_i} \,,
\end{align}
where $\boldsymbol{\gamma} \coloneqq \sum_{\pi\in\mathcal{S}_d} p_\pi \left(\pi \boldsymbol{\lambda} \right)$ are the eigenvalues of the state $\Tilde{\rho}$ which are now explicitly written as a mean over permutations of the original eigenvalues.
Therefore, the ergotropy and anti-ergotropy of the new state can be written as
\begin{align}
    \mathcal{E}^{(\hat{H})}(\tilde{\rho})
    &= E - \boldsymbol{\gamma}^\downarrow \cdot \boldsymbol{\epsilon}^\uparrow \,,\\
    \mathcal{A}^{(\hat{H})}(\tilde{\rho})
    &= \boldsymbol{\gamma}^\uparrow \cdot \boldsymbol{\epsilon}^\uparrow - E \,.
\end{align}
Now, let $\pi_\gamma^\downarrow$ be the permutation that sets the eigenvalues $\boldsymbol{\gamma}$ in decreasing order: $\pi_\gamma^\downarrow \boldsymbol{\gamma} = \boldsymbol{\gamma} ^\downarrow$.
We have that 
\begin{align}
    \mathcal{E}^{(\hat{H})}(\rho) - \mathcal{E}^{(\hat{H})}(\tilde{\rho})
    &= \boldsymbol{\gamma}^\downarrow \cdot \boldsymbol{\epsilon}^\uparrow - \boldsymbol{\lambda}^\downarrow \cdot \boldsymbol{\epsilon}^\uparrow \,,\\
    &= \left( \pi_\gamma^\downarrow \sum_{\pi\in\mathcal{S}_d} p_\pi \pi \boldsymbol{\lambda} \right) \cdot \boldsymbol{\epsilon}^\uparrow - \boldsymbol{\lambda}^\downarrow \cdot \boldsymbol{\epsilon}^\uparrow \,,\\
    &= \sum_{\pi\in\mathcal{S}_d} p_\pi \left( \pi_\gamma^\downarrow \pi \boldsymbol{\lambda} \right) \cdot \boldsymbol{\epsilon}^\uparrow - \boldsymbol{\lambda}^\downarrow \cdot \boldsymbol{\epsilon}^\uparrow \,.
\end{align}
The first term of the right-hand side is still the scalar product between the eigenvalues $\boldsymbol{\epsilon}^\uparrow$ of the Hamiltonian and a convex combination of permutations of the original spectrum $\boldsymbol{\lambda}$.
But, by construction, the term $\boldsymbol{\lambda}^\downarrow \cdot \boldsymbol{\epsilon}^\uparrow$ is already the minimum over these permutations.
Thus, we have
\begin{align}
    \mathcal{E}^{(\hat{H})}(\rho) \geq \mathcal{E}^{(\hat{H})}(\tilde{\rho}) \,.
\end{align}
Similarly, we can proceed with the anti-ergotropy such that 
\begin{align}
    \mathcal{A}^{(\hat{H})}(\rho) - \mathcal{A}^{(\hat{H})}(\Tilde{\rho})
    &= \boldsymbol{\lambda}^\uparrow \cdot \boldsymbol{\epsilon}^\uparrow - \boldsymbol{\gamma}^\uparrow \cdot \boldsymbol{\epsilon}^\uparrow \,,\\
    &= \boldsymbol{\lambda}^\uparrow \cdot \boldsymbol{\epsilon}^\uparrow - \sum_{\pi\in\mathcal{S}_d} p_\pi \left( \pi_\gamma^\uparrow \pi \boldsymbol{\lambda} \right) \cdot \boldsymbol{\epsilon}^\uparrow \geq 0 \,,
\end{align}
where the last term is positive because $\boldsymbol{\lambda}^\uparrow \cdot \boldsymbol{\epsilon}^\uparrow$ is by construction the greatest possible term in the convex sum over the permutations. Thus, we have
\begin{align}
    \mathcal{A}^{(\hat{H})}(\rho) \geq \mathcal{A}^{(\hat{H})}(\Tilde{\rho}) \,.
\end{align}
We have shown that from every state $\rho\in\sigma_E^{(\hat{H})}$ we can construct a state $\tilde{\rho}\in \Delta_E^{(\hat{H})}$ with lower ergotropy and anti-ergotropy, thus the minimum of the ergotropy (and anti-ergotropy) over the set $\sigma_E^{(\hat{H})}$ must be equal to the minimum over the set $\Delta_E^{(\hat{H})} \subset \sigma_E^{(\hat{H})}$.
\end{proof}

\subsection{\label{subsec:min-anti-passive}The minimum energy-constrained ergotropy/anti-ergotropy is always achieved by a passive/anti-passive state}

In the previous section, we showed that the energy-constrained minimum ergotropy/anti-ergotropy states at fixed mean energy are always diagonal.
We now want to further characterize these minimum states and show that they are always either passive or anti-passive states (Def.~\ref{def:anti-pass}). Note that the following proposition is equivalent to Prop.~1 of the main text.

\begin{proposition}[Prop.~1 of main text]\label{prop:minAreOrdered}
    Let $\Tilde{\rho}$ be a state of energy-constrained minimum ergotropy or anti-ergotropy, i.e., 
    \begin{align}
        &\Tilde{\rho} = \arg \min_{\rho \in \sigma_E^{(\hat{H})}} \mathcal{E}^{(\hat{H})}(\rho), \\
        &\Tilde{\rho} = \arg \min_{\rho \in \sigma_E^{(\hat{H})}} \mathcal{A}^{(\hat{H})}(\rho),
    \end{align}
    respectively.
    Then $\Tilde{\rho}$ is a passive state, $\Tilde{\rho} \in \Delta_{E,\downarrow}^{(\hat{H})}$, if $E\in[\epsilon_{\text{min}},\epsilon_{\text{mean}}]$, or an anti-passive state, $\Tilde{\rho} \in \Delta_{E,\uparrow}^{(\hat{H})}$, if $E\in[\epsilon_{\text{mean}},\epsilon_{\text{max}}]$, where $\epsilon_{\text{min}}$ is the minimum eigenvalue of $\hat{H}$, $\epsilon_{\text{max}}$ the maximum one, and $\epsilon_{\text{mean}}$ is the arithmetic mean of its eigenvalues.
\end{proposition}

\begin{proof}
We start by recalling that (see Lemma~\ref{lemma:minAreDiagonal} proof or~\cite{salvia_distribution_2021}) the ergotropy and anti-ergotropy can be written as
\begin{align}
    \forall\rho\in\sigma_E^{(\hat{H})},\quad  &\mathcal{E}^{(\hat{H})}(\rho) = E - \overbrace{\boldsymbol{\lambda}^\downarrow \cdot \boldsymbol{\epsilon}^\uparrow}^{\coloneqq E_-^{(\hat{H})}(\rho)} \,,\\
    \forall\rho\in\sigma_E^{(\hat{H})},\quad  &\mathcal{A}^{(\hat{H})}(\rho) = \overbrace{\boldsymbol{\lambda}^\uparrow \cdot \boldsymbol{\epsilon}^\uparrow}^{\coloneqq E_+^{(\hat{H})}(\rho)} - E \,,
\end{align}
where $\boldsymbol{\lambda}^\downarrow$ ($\boldsymbol{\lambda}^\uparrow$) is the spectrum of the state $\rho$ in decreasing (increasing) order and similarly $\boldsymbol{\epsilon}^\uparrow$ is the spectrum of the Hamiltonian $\hat{H}$ in increasing order.
Thus we have that minimizing the ergotropy or the anti-ergotropy corresponds to maximizing or minimizing the term $E_\pm^{(\hat{H})}(\rho)$, i.e.,
\begin{align}
    \arg \min_{\rho \in \sigma_E^{(\hat{H})}} \mathcal{E}^{(\hat{H})}(\rho) 
     &= \arg \max_{\rho \in \sigma_E^{(\hat{H})}} E_-^{(\hat{H})}(\rho)
     = \arg \overbrace{\max_{\rho \in \Delta_E^{(\hat{H})}} E_-^{(\hat{H})}(\rho)}^{\coloneqq \Tilde{E}_-^{(\hat{H})}} \,,\\
     \arg \min_{\rho \in \sigma_E^{(\hat{H})}} \mathcal{A}^{(\hat{H})}(\rho) 
     &= \arg \min_{\rho \in \sigma_E^{(\hat{H})}} E_+^{(\hat{H})}(\rho)
     = \arg \overbrace{\min_{\rho \in \Delta_E^{(\hat{H})}} E_+^{(\hat{H})}(\rho)}^{\coloneqq \Tilde{E}_+^{(\hat{H})}} \,.
\end{align}
where the second equality follows from Lemma~\ref{lemma2}.
We now reformulate the optimization over $\sigma_E^{(\hat{H})}$ as an unconstrained optimization over the full set of density matrices $\sigma(\mathcal{H})$, enforcing the energy constraint via a Lagrange multiplier.
To this end, we define the following Lagrangian functionals:
\begin{align}
   \mathcal{L}_\pm (\rho, \lambda)
   \coloneqq \mp \left( E_\pm^{(\hat{H})}(\rho) - \lambda \big( \mathrm{Tr}[\hat{H} \rho] - E \big) \right) \,,
\end{align}
where $\lambda \in \mathbb{R}$ is the Lagrange multiplier associated with the energy constraint.
The maximum or minimum energy $\tilde{E}_\pm^{(\hat{H})}$ within $\sigma_E^{(\hat{H})}$ is then obtained by solving:
\begin{align} \label{eq:lagrange}
    \tilde{E}_-^{(\hat{H})} &=
    \max_{\rho \in \sigma(\mathcal{H})} \inf_{\lambda \in \mathbb{R}} \mathcal{L}_-(\rho, \lambda) \,,\\
    \label{eq:lagrangebis} \tilde{E}_+^{(\hat{H})} &=
    \min_{\rho \in \sigma(\mathcal{H})} \sup_{\lambda \in \mathbb{R}} \mathcal{L}_+(\rho, \lambda) \,.
\end{align}
Note that the infimum and supremum over $\lambda$ precedes the maximization over $\rho$.
This ordering enforces the constraint: any state $\rho$ for which $\mathrm{Tr}[\hat{H} \rho] \neq E$ will yield $-\infty$ ($+\infty$) upon minimization (maximization) over $\lambda$, and is thus suboptimal.
In the following, we shall investigate conditions under which we can exchange the order of $\inf$ ($\sup$) and $\max$ ($\min$) in Eq.~\eqref{eq:lagrange} (Eq.~\eqref{eq:lagrangebis}).
For this purpose, we can make use of the Sion minimax theorem~\cite{sion1958minimax} (a refinement of the homonymous Von Neumann theorem~\cite{v.Neumann1928}).
Instead of presenting the theorem directly, we will state a set of sufficient conditions derived from it that justify the exchange.
\begin{enumerate} 
    \item[(i)] The set $\sigma(\mathcal{H})$ is compact and convex; the set $\mathbb{R}$ is convex as well.
    \item[(ii)] The functional $\mathcal{L}_\pm(\rho, \lambda)$ is real-valued and continuous in $\rho$ and $\lambda$.
    \item[(iii)] The functional $\mathcal{L}_\pm(\rho, \lambda)$ is concave in $\rho$ (see Lemma~\ref{prop:convErg}).
    \item[(iv)] The function $\mathcal{L}_\pm(\rho, \lambda)$ is convex in $\lambda$. This follows from linearity. 
\end{enumerate}
The conditions above are sufficient to apply the minimax theorem; we can thus write
\begin{align} \label{eq:lagrange2}
 \tilde{E}_-^{(\hat{H})}
 &= \inf_{\lambda \in \mathbb{R}} \max_{\rho \in \sigma(\mathcal{H})} \mathcal{L}_-(\rho, \lambda)
 = \inf_{\lambda \in \mathbb{R}} \max_{\rho \in \sigma(\mathcal{H})}  \big\{ E_-^{(\hat{H})}(\rho) - \lambda \big(\trace[\hat{H}\rho] - E \big) \big\} \,,\\
 \tilde{E}_+^{(\hat{H})}
 &= \sup_{\lambda \in \mathbb{R}} \min_{\rho \in \sigma(\mathcal{H})} \mathcal{L}_+(\rho, \lambda)
 = \sup_{\lambda \in \mathbb{R}} \min_{\rho \in \sigma(\mathcal{H})}  \big\{- E_+^{(\hat{H})}(\rho) + \lambda \big(\trace[\hat{H}\rho] - E \big) \big\} \,.
\end{align}
Given this, we can focus on maximizing the function $\mathcal{L}(\rho, \lambda)$. As stated in Lemma~\ref{lemma2}, we can restrict the optimisation to diagonal states.
In what follows, we represent any diagonal state by a vector whose elements are arranged in increasing order, $\bm{v} = (p_1, p_2, \ldots, p_d)$ with $p_1 \leq p_2 \leq \ldots \leq p_d$, together with an ordering $\pi \in \mathcal{S}_d$, with $\mathcal{S}_d$ being the symmetric group of degree $d$.
For each element on the diagonal, we define $\lambda_i \coloneqq \bm{v}_{\pi(i)}$, where $\bm{v} \in \Delta_d^{\uparrow}$ is the ordered probability simplex, and $\pi \in \mathcal{S}_d$ is a permutation of degree $d = \mathrm{dim}(\rho)$.
In summary: $\rho \in \Delta_E^{(\hat{H})} \leftrightarrow  \rho_{\bm{v}_\pi} : \bm{v} \in \Delta_{d}^\uparrow$. 

Then, we obtain
\begin{align}
    \max_{\rho \in \Delta_E^{(\hat{H})}} \mathcal{L}_-(\rho, \lambda) 
    &= \max_{\pi \in \mathcal{S}_d} \max_{\bm{v} \in \Delta_d^{\uparrow}} \mathcal{L}_-(\bm{v}_\pi, \lambda)
    = \max_{\bm{v} \in \Delta_d^{\uparrow}} \max_{\pi \in \mathcal{S}_d} \mathcal{L}_-(\bm{v}_\pi, \lambda) \,,\\
    \min_{\rho \in \Delta_E^{(\hat{H})}} \mathcal{L}_+(\rho, \lambda) 
    &= \min_{\pi \in \mathcal{S}_d} \min_{\bm{v} \in \Delta_d^{\uparrow}} \mathcal{L}_+(\bm{v}_\pi, \lambda)
    = \min_{\bm{v} \in \Delta_d^{\uparrow}} \min_{\pi \in \mathcal{S}_d} \mathcal{L}_+(\bm{v}_\pi, \lambda) \,,
\end{align}
where the last equality reflects the fact that the maximization can be carried out by first fixing the ordering (i.e., $\pi(1)$ is the position of the smallest element, $\pi(2)$ the second smallest, etc.), and then choosing the magnitudes of the elements in a way that preserves the ordering.
Substituting into Eqs.~\eqref{eq:lagrange} and~\eqref{eq:lagrangebis}, we obtain
\begin{align}
    \tilde{E}_-^{(\hat{H})}
    &= \inf_{\lambda \in \mathbb{R}} \max_{\rho \in \sigma(\mathcal{H})} \mathcal{L}_-(\rho, \lambda)
    = \inf_{\lambda \in \mathbb{R}} \max_{\bm{v} \in \Delta_d^{\uparrow}} \max_{\pi \in \mathcal{S}_d} \left\{ E_-^{(\hat{H})}(\rho_{\bm{v}_\pi}) - \lambda \left[\mathrm{Tr}[\hat{H} \rho_{\bm{v}_\pi}] - E \right] \right\} \,,\\
    \tilde{E}_+^{(\hat{H})}
    &= \sup_{\lambda \in \mathbb{R}} \min_{\rho \in \sigma(\mathcal{H})} \mathcal{L}_+(\rho, \lambda)
    = \sup_{\lambda \in \mathbb{R}} \min_{\bm{v} \in \Delta_d^{\uparrow}} \min_{\pi \in \mathcal{S}_d} \left\{ E_-^{(\hat{H})}(\rho_{\bm{v}_\pi}) - \lambda \left[\mathrm{Tr}[\hat{H} \rho_{\bm{v}_\pi}] - E \right] \right\} \,.
\end{align}

Focusing on the maximization and minimization over $\pi$, we exploit the fact that the first term $E_\pm^{(\hat{H})}(\rho)$ is independent of the ordering (since it is already imposed in the functional), so that we can write:
\begin{align}
    \max_{\pi \in \mathcal{S}_d} \left\{ E_-^{(\hat{H})}(\rho_{\bm{v}_\pi}) - \lambda \left[\mathrm{Tr}[\hat{H} \rho_{\bm{v}_\pi}] - E \right] \right\}
    &= - \min_{\pi \in \mathcal{S}_d} \left\{ \lambda \, \mathrm{Tr}[\hat{H} \rho_{\bm{v}_\pi}] \right\} + \lambda E + E_-^{(\hat{H})}(\rho_{\bm{v}_\mathbb{I}}) \,,\\
    \min_{\pi \in \mathcal{S}_d} \left\{ E_+^{(\hat{H})}(\rho_{\bm{v}_\pi}) + \lambda \left[\mathrm{Tr}[\hat{H} \rho_{\bm{v}_\pi}] - E \right] \right\}
    &= \min_{\pi \in \mathcal{S}_d} \left\{ \lambda \, \mathrm{Tr}[\hat{H} \rho_{\bm{v}_\pi}] \right\} - \lambda E + E_+^{(\hat{H})}(\rho_{\bm{v}_\mathbb{I}}) \,,
\end{align}
where $\pi=\mathbb{I}$ denotes the identity permutation.
The optimal state is therefore characterized by an ordering that satisfies:
\begin{align}
\tilde{\pi} = \arg \min_{\pi \in \mathcal{S}_d} \left\{ \lambda \, \mathrm{Tr}[\hat{H} \rho_{\bm{v}_\pi}] \right\} \,.
\end{align}
For any fixed Hamiltonian $\hat{H}$, the quantity $\lambda \, \mathrm{Tr}[\hat{H} \rho]$ is minimized by: passive states, when $\lambda \geq 0$, corresponding to $\tilde{\pi}(i) = i$, and anti-passive states, when $\lambda < 0$, corresponding to $\tilde{\pi}(i) = d - i$.
This proves that the states of energy-constrained minimum ergotropy and anti-ergotropy are always either passive or anti-passive states.
Since there are no passive states with energy greater than that of the completely mixed state ($\epsilon_{\text{mean}}$), and, similarly, there are no anti-passive states with energy lower than that, it follows that when $E\leq\epsilon_{\text{mean}}$ the minimum will be achieved by a passive state and when $E\geq\epsilon_{\text{mean}}$ by an anti-passive state.
\end{proof}

\subsection{\label{subsec:min-state-charac}Minimum state characterization}

We now know, thanks to Lemma~\ref{prop:minAreOrdered}, that the minimum state of both ergotropy and anti-ergotropy at fixed mean energy is either a passive state (when the energy is lower than or equal to $\epsilon_{\text{mean}}$) or an anti-passive state (when the energy is greater than or equal to $\epsilon_{\text{mean}}$).
We know that all passive states have zero ergotropy and all anti-passive states have zero anti-ergotropy.
Hence, we have non-zero energy-constrained minimum ergotropy only when $E>\epsilon_{\text{mean}}$ (i.e., when the minimum is achieved by an anti-passive state) and non-zero anti-ergotropy only when $E<\epsilon_{\text{mean}}$ (i.e., when the minimum is achieved by a passive state), as represented in Fig.~\ref{fig:anti-passive-areas}.
\begin{figure}[t]
    \centering
    \includegraphics[width=0.6\linewidth]{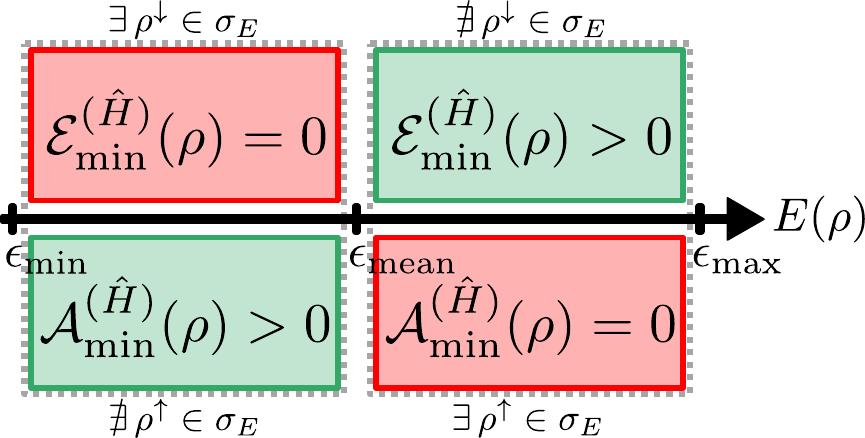}
    \caption{
        \label{fig:anti-passive-areas}
        Representation of the areas of zero and non-zero ergotropy and anti-ergotropy.
        When the mean energy of the system $E$ is lower than $\epsilon_{\text{mean}}$, passive states (which have zero ergotropy) exist but anti-passive states (which have zero anti-ergotropy) do not.
        Similarly, when the mean energy of the system $E$ is greater than $\epsilon_{\text{mean}}$, passive states do not exist but anti-passive states do.
    }
\end{figure}
The big difference is that, while \emph{all} passive states have zero ergotropy, hence with $E\leq \epsilon_{\text{mean}}$ you have \emph{many} points of minimum, usually only \emph{one} anti-passive state minimizes the ergotropy at fixed energy $E>\epsilon_{\text{mean}}$ (and similarly for the anti-ergotropy).

Here, we want to characterize these states of energy-constrained minimum ergotropy and anti-ergotropy.
In order to provide such characterization, we just need to observe that the spaces of all passive and anti-passive states (Def.~\ref{def:anti-pass-spaces}) are $(d-1)$-dimensional simplices, where $d = \dim \mathcal{H}$ is the dimension of the system's Hilbert space.
\begin{lemma}\label{lemma:simplices}
    $\Delta_{\downarrow}^{(\hat{H})}$ and $\Delta_{\uparrow}^{(\hat{H})}$ are $(d-1)$-dimensional simplices, i.e., all the states in the set can be written as a convex sum of at most $d$ basis vectors $\rho^\downarrow_k$ and $\rho_k^\uparrow$ ($k=1,\dots,d$), where $d$ is the dimension of the system and
    \begin{align}
    \label{eq:basis-passive}\rho_k^\downarrow
    &\coloneqq \frac{1}{k} \sum_{h = 1}^{k} \ket{\epsilon_h} \bra{\epsilon_h} \,,\\
    \label{eq:basis-anti-passive} \rho_k^\uparrow
    &\coloneqq \frac{1}{d+1-k} \sum_{h = k}^{d} \ket{\epsilon_h} \bra{\epsilon_h} \,.
\end{align}
\end{lemma}
\begin{proof}
    Let $\rho^\downarrow \in \Delta_{\downarrow}^{(\hat{H})}$, then, by hypothesis, we have $\rho^\downarrow = \sum_{k} \lambda_k^\downarrow \ket{\epsilon_k} \bra{\epsilon_k}$.
    The claim is that we can write it also as
    \begin{align}
        \rho^\downarrow = \sum_{k=1}^d p_k \rho_k^\downarrow \,,
    \end{align}
    where $\rho_k^\downarrow$ are the basis vectors of Eq.~\eqref{eq:basis-passive} and $p_k$ are probabilities, i.e., $p_k \geq 0$ and $\sum_k p_k = 1$.
    We can easily fix the probabilities to achieve such a result by induction.
    We start by setting $p_d \coloneqq d \cdot \lambda_d^\downarrow$, so that 
    \begin{align}
        p_d \rho_d^\downarrow
        = \lambda_d^\downarrow \sum_{h=1}^d \ket{\epsilon_h} \bra{\epsilon_h} \,.
    \end{align}
    Note that the eigenvalue of $p_d \rho_d^\downarrow$ associated to the eigenvector $\ket{\epsilon_d}$ matches the one from $\rho^\downarrow$, i.e.~$p_d \rho_d^\downarrow \ket{\epsilon_d} = \rho^\downarrow \ket{\epsilon_d}$.
    Also, the eigenvalues associated to the other eigenvectors are lower or equal to the one of $\rho^\downarrow$ ($p_d \rho_d^\downarrow \ket{\epsilon_k} \leq \rho^\downarrow \ket{\epsilon_k}$ for all $k$), since by construction $\lambda_{i+1}^\downarrow \leq \lambda_i^\downarrow$.
    Thus, we can continue by induction, setting
    \begin{align}\label{eq:probnorm-passive}
        p_{d-k} \coloneqq (d-k) \cdot (\lambda_{d-k}^\downarrow - \lambda_{d+1-k}^\downarrow) \,.
    \end{align}
    It is easy to see that, by choosing $p_{d-k}$ as in Eq.~\eqref{eq:probnorm-passive}, we have
    \begin{align}
        \left[ \sum_{h=k+1}^{d} p_h \rho_h^\downarrow
        = \sum_{h=k+1}^d \lambda_h^\downarrow \ket{\epsilon_h} \bra{\epsilon_h} + \sum_{h=1}^k \lambda_{k+1}^\downarrow \ketbra{\epsilon_h}{\epsilon_h} \right]
        \Rightarrow
        \left[ \sum_{h=k}^{d} p_h \rho_h^\downarrow
        = \sum_{h=k}^d \lambda_h^\downarrow \ket{\epsilon_h} \bra{\epsilon_h} + \sum_{h=1}^{k-1} \lambda_{k}^\downarrow \ketbra{\epsilon_h}{\epsilon_h} \right] \,.
    \end{align}
    Thus, by induction we have proved that with this basis we can construct any passive state.
    To prove that it is a simplex, we just need to show that the $p_k$ defined above are probabilities.
    Clearly, for all $k$, we have $p_k\geq0$, since $\lambda_{i+1}^\downarrow \leq \lambda_i^\downarrow$.
    Let us compute the normalization:
    \begin{align}
        \sum_{k=0}^{d-1} p_{d-k}
        &= d\cdot \lambda_d^\downarrow + \sum_{k=1}^{d-1} p_{d-k} \,,\\
        &= d\cdot \lambda_d^\downarrow + \sum_{k=1}^{d-1} (d-k) \cdot \lambda_{d-k}^\downarrow - \sum_{k=1}^{d-1} (d-k) \cdot \lambda_{d+1-k}^\downarrow \,,\\
        &= d\cdot \lambda_d^\downarrow + \sum_{k=1}^{d-1} (d-k) \cdot \lambda_{d-k}^\downarrow - \sum_{h=0}^{d-2} (d-h-1) \cdot \lambda_{d-h}^\downarrow \,,\\
        &= d\cdot \lambda_d^\downarrow + \sum_{k=1}^{d-1} (d-k) \cdot \lambda_{d-k}^\downarrow - \sum_{h=1}^{d-2} (d-h-1) \cdot \lambda_{d-h}^\downarrow - (d-1)\cdot \lambda_d^\downarrow \,,\\
        &= \sum_{k=0}^{d-1} \lambda_{d-k}^\downarrow = 1 \,.
    \end{align}
    We have thus shown that the set of passive states is a simplex generated by the given basis.
    By repeating the same steps for the anti-passive states or mapping one basis into the other, we conclude the proof.
\end{proof}

We now have all the ingredients to claim our main result about the energy-constrained minimum ergotropy and anti-ergotropy.
Note that the following theorem is equivalent to Th.~2 of the main text.
\begin{theorem}[Th.~2 of main text]\label{th:minErg} 
    Let $ \{ \sigma^\uparrow \}_E= \arg \min_{\rho \in \sigma_E^{(\hat{H})}} \mathcal{E}^{(\hat{H})}(\rho)$ be the states of minimum ergotropy at mean energy $E>\epsilon_{\text{mean}}$.
    Then, the set $\{ \sigma^\uparrow \}_E$ includes at least one state that can be written as a linear combination of at most two anti-passive states $\rho_k^\uparrow$ as defined in Eq.~\eqref{eq:basis-anti-passive}.
    Similarly, let $ \{ \sigma^\downarrow \}_E= \arg \min_{\rho \in \sigma_E^{(\hat{H})}} \mathcal{A}^{(\hat{H})}(\rho)$ be the states of minimum anti-ergotropy at mean energy $E<\epsilon_{\text{mean}}$.
    Then, the set $\{ \sigma^\downarrow \}_E$ includes at least one state that can be written as a linear combination of at most two passive states $\rho_k^\downarrow$ as defined in Eq.~\eqref{eq:basis-passive}.
\end{theorem}
The idea is that - taking ergotropy as an example - we can assume a minimum state in the set always as being anti-passive (for $E \geq \epsilon_{\text{mean}}$), thanks to Lemmas~\ref{lemma:minAreDiagonal} and~\ref{prop:minAreOrdered}.
But, thanks to Lemma~\ref{lemma:simplices} we know that those states can always be written as a convex combination of specific states in the form of Eq.~\eqref{eq:basis-anti-passive}.
But, thanks to Lemma~\ref{prop:convErg} we know that the ergotropy is convex, so the minimum can always be achieved simply by a linear combination of two of those states.
Then, to find the profile of the energy-constrained minimum ergotropy versus the mean energy, we just need to plot the points $(E_k,\mathcal{E}_k)$ for the states $\rho_k^\uparrow$ of Eq.~\eqref{eq:basis-anti-passive} ($E_k \coloneqq \trace\![\rho_k^\uparrow \hat{H}]$, $\mathcal{E}_k \coloneqq \mathcal{E}^{(\hat{H})}(\rho_k^\uparrow)$) and evaluate the convex hull, as shown in Fig.~\ref{fig:(anti)-erg-description}. 
\begin{figure}[t]
    \centering
    \includegraphics[scale=0.8]{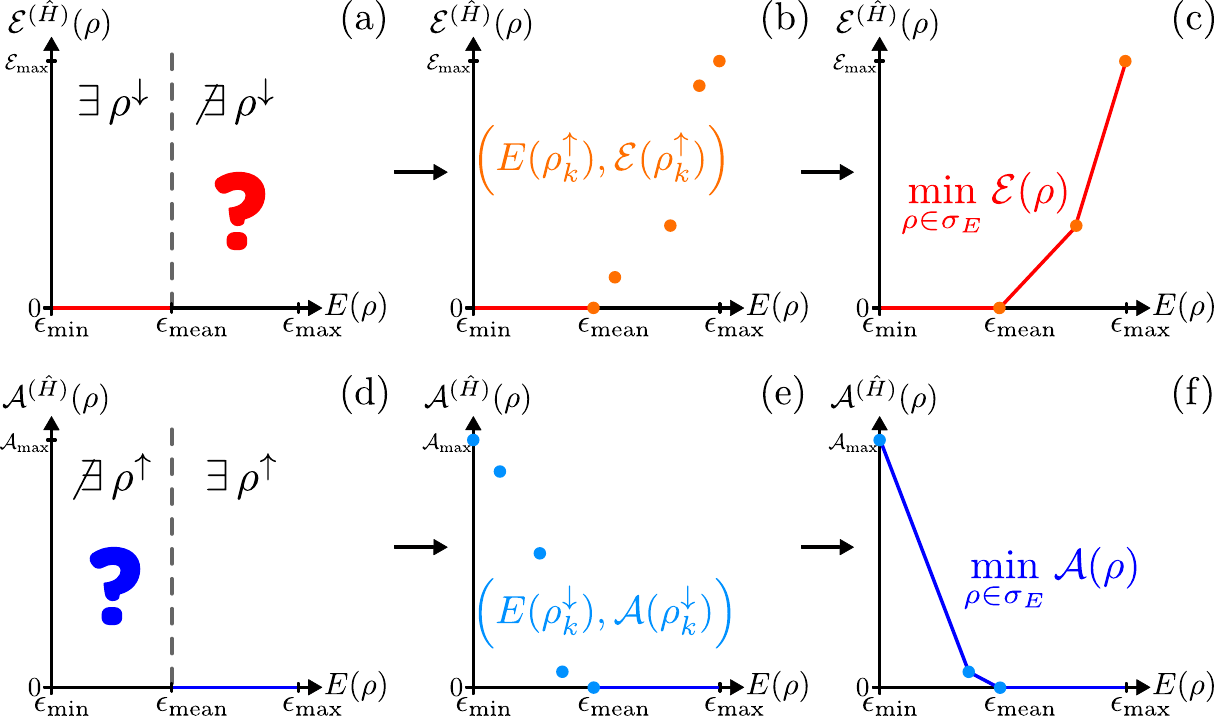}
    \caption{
    Characterization of the energy-constrained minimum ergotropy (from (a) to (c), red line) and anti-ergotropy (from (d) to (f), blue line) with respect to the mean energy.
    (a) Below $\epsilon_{\text{mean}}$ there always exist passive states; hence, the ergotropy is zero.
    (b)-(c) Above $\epsilon_{\text{mean}}$ the state of energy-constrained minimum ergotropy is either a vertex $\rho_k^\uparrow$ (orange dots) of the simplex $\Delta^\uparrow$ (Eq.~\eqref{eq:def-anti-passive-set}) or a convex combination of two of them.
    (d) Above $\epsilon_{\text{mean}}$ there always exist anti-passive states; hence, the anti-ergotropy is zero.
    (e)-(f) Below $\epsilon_{\text{mean}}$ the state of energy-constrained minimum anti-ergotropy is either a vertex $\rho_k^\downarrow$ (light-blue dots) of the simplex $\Delta^\downarrow$ (Eq.~{eq:def-passive-set}) or a convex combination of two of them.
    }
    \label{fig:(anti)-erg-description}
\end{figure}

\begin{proof}
    Let us prove the result only for the ergotropy, since the exact same steps can be repeated for the anti-ergotropy.
    Let $E>\epsilon_{\text{mean}}$.
    Thanks to Prop.~\ref{prop:minAreOrdered} we know that the energy-constrained minimum ergotropy is always achieved by an anti-passive state, hence,
    \begin{align}
        \mathcal{E}_{\text{min}}^{(\hat{H})}(E)
        &= \min_{\rho\in\Delta_{E,\uparrow}^{(\hat{H})}} \mathcal{E}^{(\hat{H})}(\rho) \,.
    \end{align}
    It follows that, thanks to Lemma~\ref{lemma:simplices}, every state in the set can be written as a convex combination of the states $\rho_k^\uparrow$ of Eq.~\eqref{eq:basis-anti-passive}.
    We now recall that the ergotropy and anti-ergotropy are linear with respect to passive and anti-passive states.
    This happens because all passive and anti-passive states are optimally charged and discharged by the same unitary $\hat{V} \coloneqq \sum_{k=1}^d \ketbra{\epsilon_{d+1-k}}{\epsilon_k}$.
    It follows that the minimization problem can be rewritten as
    \begin{align}
        \mathcal{E}_{\text{min}}^{(\hat{H})}(E)
        &= \min_{\boldsymbol{p},\, \boldsymbol{p}\cdot \boldsymbol{E} = E} \boldsymbol{p} \cdot \boldsymbol{\mathcal{E}} \,,
    \end{align}
    where $\boldsymbol{p}$ is a probability distribution, $(\boldsymbol{E})_k \coloneqq \trace\!\left[ \hat{H} \rho_k^\uparrow \right]$ and $(\boldsymbol{\mathcal{E}})_k \coloneqq \mathcal{E}^{(\hat{H})}(\rho_k^\uparrow)$ are respectively the energy and ergotropy of the vertices of the simplex $\Delta_\uparrow^{(\hat{H})}$. 
    
    This is a linear program, and we now want to show that the minimization can always be achieved by either a vertex ($(\boldsymbol{p})_k = 0$ for all $k$ but one) or a convex combination of two vertices ($(\boldsymbol{p})_k = 0$ for all $k$ but two).
    Let $\boldsymbol{p}^* \in \arg \min \boldsymbol{p} \cdot \boldsymbol{\mathcal{E}}$ be an optimal solution for a given mean energy value $E\in[\epsilon_{\text{mean}},\epsilon_{d}]$.
    Let $\boldsymbol{p}_{k_j}^* > 0$ for $j=1,\dots,s$ ($1\leq s \leq d$) be the non-zero entries of the vector $\boldsymbol{p}^*$.
    Assume now that $s>2$, i.e., the optimal solution found is a convex combination of at least three different vertexes.
    We argue that in this case the minimum is also achieved by any convex combination having as non-zero entries only two indices $a,b \in \{ k_j \}_j$ (such that $E_a < E < E_b$, so that the energy constraint can be satisfied).
    To prove this, let $h \in \{ k_j \}_j$ such that $k_1 < h < k_s$.
    Consider the probability distribution $\boldsymbol{q}$,
    \begin{align}
        \boldsymbol{q} = \boldsymbol{p}^* + \delta \boldsymbol{t}^{(h)} \,,
    \end{align}
    where $\boldsymbol{t}^{(h)}$ has entries $\boldsymbol{t}^{(h)}_h = -1$, $\boldsymbol{t}^{(h)}_{k_1} = t_h$, $\boldsymbol{t}^{(h)}_{k_s} = 1 - t_h$, and zero otherwise, with
    \begin{align}
        t_h = \frac{E_{k_s} - E_{h}}{E_{k_s}-E_{k_1}} \,,
    \end{align}
    so that $\forall \delta$ the vector $\boldsymbol{q}$ also satisfies the energy constraint.
    Note that $\forall \delta$ we also have that $\sum_{i} \boldsymbol{q}_i = 1$, but there may be negative entries.
    To prevent this, we will also assume that $\delta\in(-\sigma,\sigma)$ for $\sigma\ll1$, so that the vector $\boldsymbol{q}$ is guaranteed to be a probability distribution and hence a possible solution to the minimum problem.
    We argue that $\boldsymbol{q}$ is also a solution to the minimum problem $\forall \delta$ feasible.
    We have
    \begin{align}
        \boldsymbol{q} \cdot \boldsymbol{\mathcal{E}}
        &= \boldsymbol{p}^* \cdot \boldsymbol{\mathcal{E}}
            + \delta \overbrace{\left( t_h \boldsymbol{\mathcal{E}}_{k_1} - \boldsymbol{\mathcal{E}}_h + (1-t_h) \boldsymbol{\mathcal{E}}_{k_s} \right)}^{ \eqqcolon \Delta \mathcal{E}} \,,\\
        &\geq \boldsymbol{p}^* \cdot \boldsymbol{\mathcal{E}} \,,
    \end{align}
    where the inequality is a consequence of $\boldsymbol{p}^*$ being an optimal solution.
    Since $\delta$ can be both positive and negative, it must be $\Delta \mathcal{E} = 0$.
    This proves that $\boldsymbol{q} \cdot \boldsymbol{\mathcal{E}}$ is also an optimal solution.
    By choosing $\delta = \boldsymbol{p}^*_h$ for all $h$ such that $k_1 < h\in\{k_j\}_j < k_s$, I can thus eliminate all non-zero entries but $k_1,k_s$, and obtain an optimal vector that has only two non-zero components.
\end{proof}

\subsection{\label{subsec:anti-h-min-erg}Anti-symmetric Hamiltonians}

Thanks to Theorem~\ref{th:minErg} we now know that usually the state of energy-constrained minimum ergotropy (anti-ergotropy), depending on the mean energy, is either \emph{any} passive state (anti-passive state) or \emph{a specific} anti-passive state (passive state) that can be written as a linear combination of two states.
There is a special scenario in which all the anti-passive (passive) states at fixed mean energy have the same ergotropy (anti-ergotropy), hence being all points of energy-constrained minimum ergotropy (anti-ergotropy).
\begin{definition}\label{def:anti-symm-h}
    Let $\hat{H} = \sum_{k=1}^d \epsilon_k \ket{\epsilon_k} \bra{\epsilon_k}$ be a finite-dimensional Hamiltonian ($d<\infty$) and let us assume without loss of generality that the eigenvalues are ordered, i.e., $\epsilon_{k+1} \geq \epsilon_k$. Thus the Hamiltonian is \textbf{antisymmetric} if and only if the sum of oppositely ordered eigenvalues always has the same value, i.e.,
    \begin{align}
        \exists c\in\mathbb{R} :
        \forall \, k\,, \,\epsilon_{k} + \epsilon_{d+1-k} = c \,.
    \end{align}
\end{definition}
Common examples of these Hamiltonians are the angular momentum $\hat{H} = \hat{J}_z$ or the $N$ qubits Hamiltonian, $\hat{H} = \sum_{k=1}^N \omega_k \hat{\sigma}_k^z$, where $\omega_k$ is the energy gap between the ground and excited state of the qubit $k$ and $\hat{\sigma}_k^z$ is the Pauli matrix in the $z$-direction for the qubit $k$ tensor the identity for the other ones.
For this class of Hamiltonians, the following result holds, which is equivalent to the energy-constrained minimum ergotropy and anti-ergotropy results of Th.~3 of the main text.
\begin{lemma}[Part of Th.~3 of main text]\label{lemma:min-anti-erg-anti-h}
    Let $\hat{H}_{\text{as}}$ be an antisymmetric Hamiltonian.
    Then, we have that
    \begin{align}
        \mathcal{E}_{\text{min}}^{(\hat{H}_{\text{as}})}(E)
        &= \begin{cases}
            0 & \text{ if }E\leq\epsilon_{\text{mean}} \,,\\
            2(E-\epsilon_{\text{mean}}) & \text{ if }E\geq\epsilon_{\text{mean}} \,,
        \end{cases} \\
        \mathcal{A}_{\text{min}}^{(\hat{H}_{\text{as}})}(E)
        &= \begin{cases}
            2(\epsilon_{\text{mean}}-E) & \text{ if }E\leq\epsilon_{\text{mean}} \,,\\
            0 & \text{ if }E\geq\epsilon_{\text{mean}} \,.
        \end{cases}
    \end{align}
    where $\epsilon_{\text{mean}} \equiv (\epsilon_{\text{min}}+\epsilon_{\text{max}})/2$ is the maximum energy gap between two different energy levels.
    Also, we have that all anti-passive (passive) states having the same energy $\rho^\uparrow \in \Delta^{(\hat{H}_{\text{as}})}_{E,\uparrow}$ ($\rho^\downarrow \in \Delta^{(\hat{H}_{\text{as}})}_{E,\downarrow}$) have the same ergotropy (anti-ergotropy), hence equal to the minimum.
\end{lemma}
This result is due to the \emph{alignment} of the vertex of the simplices with respect to the figure of merit, as represented in Fig.~\ref{fig:anti-h-min-erg-anti-erg}.
\begin{figure}[t]
    \centering
    \includegraphics[scale=0.8]{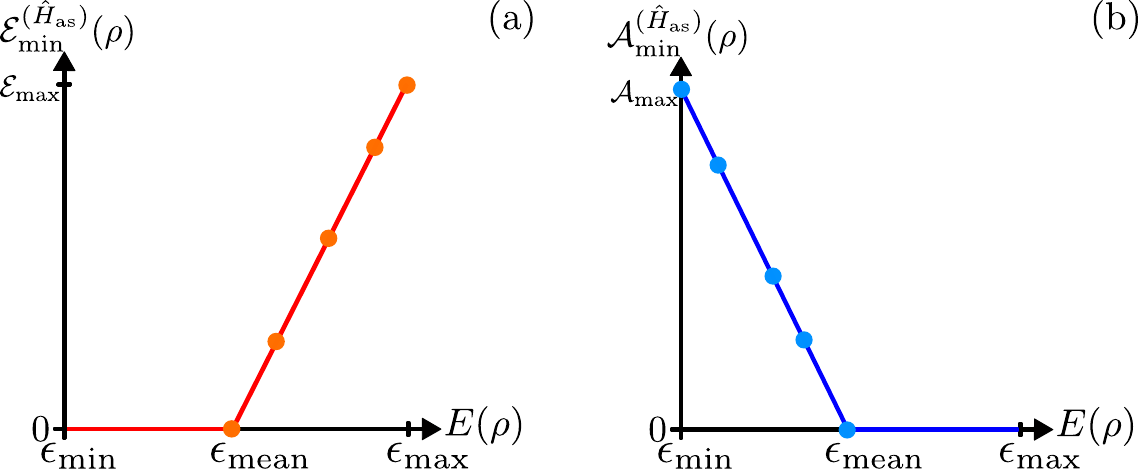}
    \caption{Representation of the energy-constrained minimum ergotropy (a) (red line) and anti-ergotropy (b) (blue line) with respect to the mean energy when the Hamiltonian is anti-symmetric (Def.~\ref{def:anti-symm-h}). The orange dots represent the vertices of the simplex of anti-passive states, while the light-blue dots represent the vertices of the simplex of passive states.}
    \label{fig:anti-h-min-erg-anti-erg}
\end{figure}
\begin{proof}
    The proof follows trivially from the definition of anti-symmetric Hamiltonian, the linearity of ergotropy and anti-ergotropy with respect to passive and anti-passive states, and Prop.~\ref{prop:minAreOrdered}.
    In this special case, though, we can easily arrive at the same result by simply exploiting Lemma~\ref{lemma:minAreDiagonal}, i.e., just knowing that the states of energy-constrained minimum ergotropy and anti-ergotropy are diagonal.
    We know that a state $\tilde{\rho}$ of energy-constrained minimum ergotropy or anti-ergotropy is diagonal with respect to the target anti-symmetric Hamiltonian $\hat{H}_{\text{as}} = \sum_{k=1}^d \epsilon_k \ketbra{\epsilon_k}{\epsilon_k}$, $\tilde{\rho} = \sum_k \lambda_k \ketbra{\epsilon_k}{\epsilon_k}$.
    As usual, we will assume without loss of generality that the eigenvalues of the Hamiltonian are already ordered, $\epsilon_k \leq \epsilon_{k+1}$.
    Thus, the mean energy of the state $\tilde{\rho}$ is simply $E = \boldsymbol{\lambda} \cdot \boldsymbol{\epsilon}^\uparrow$.
    
    By exploiting the characterization of the ergotropy and the anti-symmetry of the Hamiltonian, we have
    \begin{align}
        \mathcal{E}^{(\hat{H}_{\text{as}})} (\tilde{\rho})
        &= E - \boldsymbol{\lambda}^\downarrow \cdot \boldsymbol{\epsilon}^\uparrow
        = E - \boldsymbol{\lambda}^\uparrow \cdot \boldsymbol{\epsilon}^\downarrow \,,\\
        &= E - \sum_{k=1}^d \lambda_k^\uparrow \epsilon_{k}^\downarrow \,,\\
        &= E - \sum_{k=1}^d \lambda_k^\uparrow \left( 2\epsilon_{\text{mean}} -  \epsilon_{d+1-k}^\downarrow \right) \,,\\
        &= E - 2\epsilon_{\text{mean}} + \sum_{k=1}^d \lambda_k^\uparrow \epsilon_{k}^\uparrow \,,\\
        &= E - 2\epsilon_{\text{mean}} + \boldsymbol{\lambda}^\uparrow \cdot \boldsymbol{\epsilon}^\uparrow \,,\\
        &\geq E - 2\epsilon_{\text{mean}} + E = 2E - 2\epsilon_{\text{mean}} \,,
    \end{align}
    where in the last step we exploited that $\boldsymbol{\lambda}^\uparrow \cdot \boldsymbol{\epsilon}^\uparrow \geq \boldsymbol{\lambda} \cdot \boldsymbol{\epsilon}^\uparrow = E$.
    But this lower bound is always saturated if the state $\tilde{\rho}$ is anti-passive, hence the proof for the ergotropy.
    The same steps can be repeated for the anti-ergotropy, finishing the proof.
\end{proof}
Antisymmetric Hamiltonians have other important properties, which will be discussed in Sec.~\ref{subsec:anti-h-ext-energy}.

\section{\label{sec:algo}An efficient algorithm to evaluate the energy-constrained minimum ergotropy}

In this section, we provide algorithms (here written in Python code) to efficiently evaluate the energy-constrained minimum ergotropy, according to the results of Theorem~\ref{th:minErg}.
The same algorithms can be easily modified to find the energy-constrained minimum anti-ergotropy.
Let $d \coloneqq \text{dim}(\mathcal{H})$ be the dimension of the system of interest.
We can find the points of energy-constrained minimum ergotropy (Fig.~\ref{fig:(anti)-erg-description}~(c), light-red points) in $O(d^2)$ steps.
First, we evaluate all the mean energies and ergotropies  $(E(\rho_k^\uparrow),\mathcal{E}(\rho_k^\uparrow))$ for the basis $\{\rho_k^\uparrow\}_{k=1\dots,d}$ of the anti-passive states (i.e., we find all the light-red points in Fig.~\ref{fig:(anti)-erg-description}~(b)), as defined in Eq.~\eqref{eq:basis-anti-passive}.
In the algorithm, such values are saved in the Python lists \texttt{critEnergies} and \texttt{critErgotropies}.
Afterwards, between those points, we want to select the minimum ones, which will be saved in the lists \texttt{minEnergies} and \texttt{minErgotropies}.
We already know that the first element in such lists will be given by the energy ($\epsilon_{\text{mean}}$) and ergotropy (zero) of the completely mixed state.
We can then easily find the next element by evaluating the angular coefficients \texttt{testm} between the last element found and all the remaining points and choosing the smaller one.
This can be done with two iterations inside one another, hence the complexity $O(d^2)$.

\begin{mintedbox}{python}
    import numpy as np
    
    def minErgPoints(hspectrum):
        """
        Compute the energy-constrained minimum ergotropy curve from an energy spectrum.
    
        Parameters:
            hspectrum (List[float] or np.ndarray): The energy spectrum (assumed sorted ascending).
    
        Returns:
            Tuple[np.ndarray, np.ndarray]: Arrays of minimal ergotropy values and associated mean energies.
        """
        hspectrum = np.asarray(hspectrum)
        dimension = len(hspectrum)
        # Evaluate mean energy and ergotropy for the basis of anti-passive states.
        critEnergies = []
        critErgotropies = []
        for k in range(dimension):
            upperAvg = np.sum(hspectrum[k:]) / (dimension - k)
            lowerAvg = np.sum(hspectrum[:dimension - k]) / (dimension - k)
            critEnergies.append(upperAvg)
            critErgotropies.append(upperAvg - lowerAvg)
        # Find the points of energy-constrained minimum ergotropy by comparing angular coefficients.
        minEnergies = [critEnergies[0]]
        minErgotropies = [critErgotropies[0]]
        k = 0
        while k < dimension - 1:
            h = k + 1
            m = (critErgotropies[h] - minErgotropies[-1]) / (critEnergies[h] - minEnergies[-1])
            while h < dimension:
                testm = (critErgotropies[h] - minErgotropies[-1]) / (critEnergies[h] - minEnergies[-1])
                if testm <= m:
                    m = testm
                    k = h
                h += 1
            minEnergies.append(critEnergies[k])
            minErgotropies.append(critErgotropies[k])
        return np.array(minEnergies), np.array(minErgotropies)
\end{mintedbox}

Once you have found the points of energy-constrained minimum ergotropy $\{(E_k, \mathcal{E}_k)\}_{k=1,\dots,s}$ ($s\leq d$), we can find the energy-constrained minimum ergotropy associated to any value of the mean energy $E$ in $O(s)$ steps.
First, we find the index $a$ such that $E_a \leq E \leq E_{a+1}$, an operation that requires at most $O(s)$ steps.
We continue by evaluating the probability $p\in[0,1]$ such that $E = pE_a + (1-p) E_{a+1}$.
The energy-constrained minimum ergotropy associated with $E$ will simply be $\mathcal{E}_{\text{min}}^{(\hat{H})}(E) = p \mathcal{E}_a + (1-p)\mathcal{E}_{a+1}$.
\begin{mintedbox}{python}
    import numpy as np

    def minErg(energy, hspectrum=None, minEnergies=None, minErgotropies=None):
        """
        Compute the energy-constrained minimum ergotropy associated with a given input energy using precomputed
        or derived minimal ergotropy curve points.
    
        Parameters:
            energy (float): The input energy value for which to evaluate minimal ergotropy.
            hspectrum (Optional[List[float] or np.ndarray]): Hamiltonian spectrum, used if minimal curve is not given.
            minEnergies (Optional[np.ndarray]): Array of minimal energy values from the convex ergotropy curve.
            minErgotropies (Optional[np.ndarray]): Array of corresponding minimal ergotropies.
    
        Returns:
            float: The energy-constrained minimum ergotropy corresponding to the given energy.
    
        Raises:
            ValueError: If neither hspectrum nor (minEnergies and minErgotropies) are provided.
            ValueError: If energy is out of the range covered by minEnergies.
        """
        # Validate or compute minimal energy/ergotropy curve
        if minEnergies is None or minErgotropies is None:
            if hspectrum is None:
                raise ValueError("You must provide either hspectrum or both minEnergies and minErgotropies.")
            minEnergies, minErgotropies = minErgPoints(hspectrum)
        minEnergies = np.asarray(minEnergies)
        minErgotropies = np.asarray(minErgotropies)
        # Check if given energy is within bounds
        if energy < minEnergies[0] or energy > minEnergies[-1]:
            raise ValueError(f"Input energy {energy} is out of bounds of the minimum energy range "
                             f"[{minEnergies[0]}, {minEnergies[-1]}].")
        # Find the segment in which the energy lies
        for k in range(len(minEnergies) - 1): 
            if E1 <= minEnergies[k]:
                p = (minEnergies[k+1] - energy) / (minEnergies[k+1] - minEnergies[k])
                erg = p * minErgotropies[k] + (1 - p) * minErgotropies[k + 1]
                return erg
\end{mintedbox}

\section{\label{sec:implications}An upper bound for the coherent ergotropy}

A consequence of the characterization of the energy-constrained minimum ergotropy with respect to the mean energy is an optimal upper bound for the coherent ergotropy with respect to the same figure of merit - and similarly for the anti-ergotropy.
We recall that the coherent ergotropy~\cite{PhysRevLett.125.180603} $\mathcal{E}_c^{(\hat{H})}(\rho)$ of a state is defined as the difference between its ergotropy and the ergotropy of the dephased state $\Delta(\rho) \coloneqq \sum_k \braket{\epsilon_k | \rho | \epsilon_k} \ketbra{\epsilon_k}{\epsilon_k}$,
\begin{align}
    \mathcal{E}_c^{(\hat{H})}(\rho)
    \coloneqq \mathcal{E}^{(\hat{H})}(\rho) - \mathcal{E}^{(\hat{H})}(\Delta(\rho)) \,.
\end{align}
This function quantifies the energetic contribution of the coherences of the state, or, equivalently, how much extractable energy you \emph{cannot} extract if you can perform only incoherent operations (i.e. permutations of the energy levels) instead of any unitary~\cite{PhysRevLett.125.180603}.
Although not discussed in the literature, in the same spirit, we can define the coherent anti-ergotropy,
\begin{align}
    \mathcal{A}_c^{(\hat{H})}(\rho)
    \coloneqq \mathcal{A}^{(\hat{H})}(\rho) - \mathcal{A}^{(\hat{H})}(\Delta(\rho)) \,.
\end{align}

Thanks to our characterization of the energy-constrained minimum ergotropy and anti-ergotropy, we know that the states of minima can always be chosen diagonal; hence, we can prove the following (as illustrated in Fig.~\ref{fig:coherent-bound})
\begin{figure}[t]
    \centering
    \includegraphics[scale=0.8]{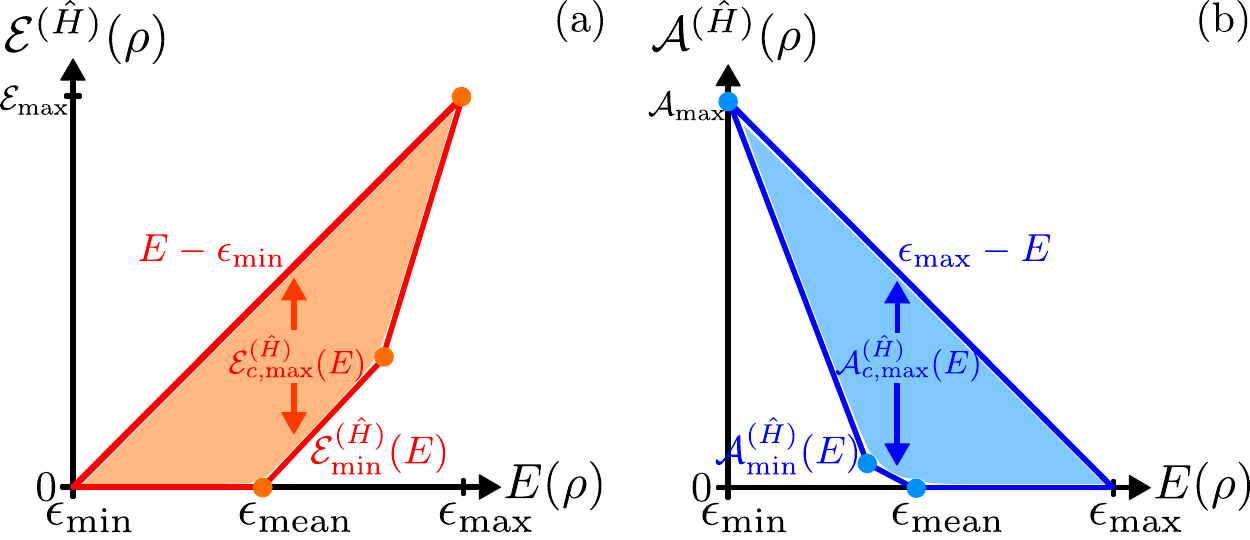}
    \caption{Description of the maximum coherent ergotropy (a) and anti-ergotropy (b) at fixed mean energy.
    The maximum coherent ergotropy (a) is given by the difference between the maximum ergotropy -- equal to the mean energy $E$ minus the ground state energy $\epsilon_{\text{min}}$ -- and the energy-constrained minimum ergotropy $\mathcal{E}_{\text{min}}^{(\hat{H})}(E)$.
    Similarly, the maximum coherent anti-ergotropy (b) is given by the difference between the maximum anti-ergotropy -- equal to the maximum energy $\epsilon_{\text{max}}$ minus the mean energy $E$ -- and the energy-constrained minimum anti-ergotropy $\mathcal{A}_{\text{min}}^{(\hat{H})}(E)$.}
    \label{fig:coherent-bound}
\end{figure}
\begin{lemma}
    The maximum coherent ergotropy $\mathcal{E}_{c,\text{max}}^{(\hat{H})}(E)$ and anti-ergotropy $\mathcal{A}_{c,\text{max}}^{(\hat{H})}(E)$ with respect to the set $\rho\in\sigma_E^{(\hat{H})}$ of all states at fixed mean energy $E$ are respectively equal to
    \begin{align}
        \mathcal{E}_{c,\text{max}}^{(\hat{H})}(E)
        &\coloneqq \max_{\rho\in\sigma_E^{(\hat{H})}} \mathcal{E}_c^{(\hat{H})}(\rho) \,,\\
        &= E - \epsilon_{\text{min}} - \mathcal{E}_{\text{min}}^{(\hat{H})}(E) \,,\\
        \mathcal{A}_{c,\text{max}}^{(\hat{H})}(E)
        &\coloneqq \max_{\rho\in\sigma_E^{(\hat{H})}} \mathcal{A}_c^{(\hat{H})}(\rho) \,,\\
        &= \epsilon_{\text{max}} - E - \mathcal{A}_{\text{min}}^{(\hat{H})}(E) \,.
    \end{align}
\end{lemma}
\begin{proof}
    The proof follows easily thanks to Lemma~\ref{lemma:minAreDiagonal}.
    We have
    \begin{align}
        \mathcal{E}_{c,\text{max}}^{(\hat{H})}(E)
        &= \max_{\rho\in\sigma_E^{(\hat{H})}} \left[ \mathcal{E}^{(\hat{H})}(\rho) - \mathcal{E}^{(\hat{H})}(\Delta(\rho)) \right] \,,\\
        &\leq \max_{\rho\in\sigma_E^{(\hat{H})}} \mathcal{E}^{(\hat{H})}(\rho)  - \min_{\rho\in\sigma_E^{(\hat{H})}} \mathcal{E}^{(\hat{H})}(\Delta(\rho)) \,,\\
        &= E - \epsilon_{\text{min}} -\mathcal{E}_{\text{min}}^{(\hat{H})}(E) \,,
    \end{align}
    where in the last step we exploited the fact that the state that minimizes the ergotropy is already diagonal, hence the minimum of the dephased state is equal to the minimum of all states.
    Note also that we used the equality
    \begin{align}
        \max_{\rho\in\sigma_E^{(\hat{H})}} \mathcal{E}^{(\hat{H})}(\rho)
        &= E - \min_{\rho\in\sigma_E^{(\hat{H})}} \boldsymbol{\lambda^\downarrow}(\rho) \cdot \boldsymbol{\epsilon^\uparrow} \,,\\
        &= E - \epsilon_{\text{min}} \,,
    \end{align}
    where $\boldsymbol{\lambda^\downarrow}(\rho)$ is the decreasingly ordered spectrum of the state $\rho$.
    Now, let $\sigma_E^{(\hat{H})} \ni \tilde{\rho} = \sum_k \lambda_k \ketbra{\epsilon_k}{\epsilon_k} $ be a state of energy-constrained minimum ergotropy.
    One can easily see that the inequality is saturated by taking as input state the pure state $\ket{\Psi}\bra{\Psi}$, where $\ket{\Psi} = \sum_k \sqrt{\lambda_k} \ket{\epsilon_k}$.
    
    Similarly, for the anti-ergotropy, we get
    \begin{align}
        \mathcal{A}_{c,\text{max}}^{(\hat{H})}(E)
        &= \max_{\rho\in\sigma_E^{(\hat{H})}} \left[ \mathcal{A}^{(\hat{H})}(\rho) - \mathcal{A}^{(\hat{H})}(\Delta(\rho)) \right] \,,\\
        &\leq \max_{\rho\in\sigma_E^{(\hat{H})}} \mathcal{A}^{(\hat{H})}(\rho)  - \min_{\rho\in\sigma_E^{(\hat{H})}} \mathcal{A}^{(\hat{H})}(\Delta(\rho)) \,,\\
        &= \epsilon_{\text{max}} - E - \mathcal{E}_{\text{min}}^{(\hat{H})}(E) \,,
    \end{align}
    which is saturated by taking the state $\ketbra{\Psi}{\Psi}$, where $\ket{\Psi} = \sum_k \sqrt{\sigma_k} \ket{\epsilon_k}$ and $\sigma_E^{(\hat{H})} \ni \tilde{\rho} = \sum_k \sigma_k \ketbra{\epsilon_k}{\epsilon_k}$ is a state of energy-constrained minimum anti-ergotropy.
\end{proof}

\section{\label{sec:unknown-ext}Max-WCEE and max-WCIE properties}

So far we have provided a complete characterization of the energy-constrained minimum ergotropy and anti-ergotropy for \emph{any} finite-dimensional Hamiltonian.
In order to extract or charge the maximum amount of energy, though, a specific (potentially not unique) state-dependent unitary $\hat{U}_{\max}^{(\pm,\rho)} = \arg \max_{\Lambda\in\mathcal{U}} \left[ \pm \Delta E^{(\hat{H})} (\rho,\Lambda) \right]$ is needed.
Let $\rho = \sum_k \lambda_k \ket{\phi_k} \bra{\phi_k}$ be the spectral decomposition of the target state, with $\lambda_{k+1} \leq \lambda_k$.
The unitary used to extract (charge) the maximum amount of energy is $\hat{U}_{\max}^{(+,\rho)} = \sum_k \ket{\epsilon_k} \bra{\phi_k}$ ($\hat{U}_{\max}^{(-,\rho)} = \sum_k \ket{\epsilon_{d+1-k}} \bra{\phi_k}$), where $\hat{H} = \sum_{k=1}^d \epsilon_k \ketbra{\epsilon_k}{\epsilon_k}$ is the Hamiltonian of the system (and, as usual, the eigenvalues are increasingly ordered, $\epsilon_k \leq \epsilon_{k+1}$ for all $k$).
This unitary requires almost full knowledge of the state in order to be implemented and may vary considerably from one state to another.

We now want to characterize the \emph{minimum} amount of energy $\tilde{\mathcal{E}}^{(\hat{H})}(\mathcal{O})$ ($\tilde{\mathcal{A}}^{(\hat{H})}(\mathcal{O})$) that can be safely extracted (charged) from a state $\rho$ when the state itself is unknown but some information $\mathcal{O}(\rho)$ on it is known.
Also, we want to characterize the optimal unitary $\hat{U}_{\max}^{(\pm,\mathcal{O})}$ that needs to be used to extract or inject energy into the system.
In what follows, we will take $\mathcal{O}(\rho) \equiv E(\rho) \coloneqq \trace \left[ \rho \hat{H} \right]$, i.e., we will assume that the only information available on the initial state is its mean energy.
\begin{definition}
    The \textbf{maximum worst-case extractable (injectable) energy}, max-WCEE $\tilde{\mathcal{E}}^{(\hat{H})}(E)$ (max-WCIE $\tilde{\mathcal{A}}^{(\hat{H})}(E)$), when $E \equiv E(\rho)$ is the only information available, is defined to be the optimal energy you can extract (charge) through unitary operations \emph{after} taking the minimization with respect to all possible states having mean energy $E$ (i.e., the worst-case scenario).
    \begin{align}
        \tilde{\mathcal{E}}^{(\hat{H})} (E) &\coloneqq \max_{\Lambda \in \mathcal{U}} \min_{\rho \in \sigma_E^{(\hat{H})}} \left[ \Delta E^{(\hat{H})} (\rho,\Lambda) \right] \,,\\
        \tilde{\mathcal{A}}^{(\hat{H})} (E) &\coloneqq \max_{\Lambda \in \mathcal{U}} \min_{\rho \in \sigma_E^{(\hat{H})}} \left[ - \Delta E^{(\hat{H})} (\rho,\Lambda) \right] \,,
    \end{align}
    where the minimum $\min_{\rho \in \sigma_E^{(\hat{H})}} \left[ \pm \Delta E^{(\hat{H})} (\rho,\Lambda) \right]$ is intended to be with respect to the fixed and arbitrary quantum channel $\Lambda$.
\end{definition}

Characterizing these functionals is not a simple task.
Luckily, since the $\max-\min$ is lower or equal to the $\min-\max$~\cite{Boyd_Vandenberghe_2004}, we have already found optimal upper bounds for these quantities.
\begin{align}
    \tilde{\mathcal{E}}^{(\hat{H})} (E)
    &= \max_{\Lambda \in \mathcal{U}} \min_{\rho \in \sigma_E^{(\hat{H})}} \left[ \Delta E^{(\hat{H})} (\rho,\Lambda) \right] \,,\\
    &\leq \min_{\rho \in \sigma_E^{(\hat{H})}} \max_{\Lambda \in \mathcal{U}} \left[ \Delta E^{(\hat{H})} (\rho,\Lambda) \right] = \mathcal{E}_{\text{min}}^{(\hat{H})}(E) \,,\\
    \tilde{\mathcal{A}}^{(\hat{H})} (E)
    &= \max_{\Lambda \in \mathcal{U}} \min_{\rho \in \sigma_E^{(\hat{H})}} \left[ - \Delta E^{(\hat{H})} (\rho,\Lambda) \right] \,,\\
    &\leq \min_{\rho \in \sigma_E^{(\hat{H})}} \max_{\Lambda \in \mathcal{U}} \left[ - \Delta E^{(\hat{H})} (\rho,\Lambda) \right] = \mathcal{A}_{\text{min}}^{(\hat{H})}(E) \,.
\end{align}
Note that, like the ergotropy and anti-ergotropy, these are positive semi-definite functions.
It is clear then that when the mean energy is lower (greater) or equal to the energy of the completely mixed state $\epsilon_{\text{mean}}$, since the ergotropy (anti-ergotropy) is already zero, you cannot safely extract (charge) any energy from a state without further information on it.

These inequalities are in general strict, but there are some special cases in which these two quantities have the same values.
In Sections~\ref{subsec:anti-h-ext-energy},~\ref{subsec:diag}, and~\ref{subsec:rand} we will discuss several important special cases in which these upper bounds can be saturated.
These cases will show us a path towards some practical unitaries $\hat{U}_{\max}^{(\pm,E)}$ that are not in general optimal but can guarantee good results.
Finally, exploiting one of these unitaries, in Sec.~\ref{subsec:lowerbound} we will derive a non-optimal lower bound for the almost unknown extractable and chargeable energy to ensure its feasibility.

\subsection{\label{subsec:anti-h-ext-energy}Anti-symmetric Hamiltonians}

The first very important case in which we can saturate the upper bound is the nature-ubiquitous scenario of anti-symmetric Hamiltonians.
In this case, not only can we always extract at least the energy-constrained minimum ergotropy $\mathcal{E}_{\text{min}}^{(\hat{H})}(E)$, but -- when the mean energy exceeds $\epsilon_{\text{mean}}$ -- there exists a single energy-independent unitary that guarantees the extraction of exactly that amount from all states (and similarly for the anti-ergotropy).
This can be summarised with the following statement, equivalent to the max-WCEE and max-WCIE results of Th.~3 of the main text.

\begin{theorem}[Part of Th.~3 of main text]
    Let $\hat{H}_{\text{as}} = \sum_{k=1}^d \epsilon_k \ketbra{\epsilon_k}{\epsilon_k}$ be an anti-symmetric Hamiltonian (Def.~\ref{def:anti-symm-h}).
    We then have that the almost unknown extractable and chargeable energy is equal to the energy-constrained minimum ergotropy and anti-ergotropy, i.e.,
    \begin{align}
        \tilde{\mathcal{E}}^{(\hat{H})} (E)
        &= \mathcal{E}_{\text{min}}^{(\hat{H})}(E) \,,\\
        \tilde{\mathcal{A}}^{(\hat{H})} (E)
        &= \mathcal{A}_{\text{min}}^{(\hat{H})}(E) \,.
    \end{align}
    Furthermore, let $\hat{U}_{\text{rev}}^{(\pm,E)}$ be the unitary that reverses the populations above or below the threshold $E=\epsilon_{\text{mean}}$,
    \begin{align}
        \hat{U}_{\text{rev}}^{(+,E)}
        &\coloneqq \begin{cases}
            \hat{\mathbb{I}} & E \leq \epsilon_{\text{mean}} \,,\\
            \hat{U}_{\text{rev}} \coloneqq \sum_{k=1}^d \ketbra{\epsilon_{d+1-k}}{\epsilon_k} & E \geq \epsilon_{\text{mean}} \,,
        \end{cases} \\
        \hat{U}_{\text{rev}}^{(-,E)}
        &\coloneqq \begin{cases}
            \hat{U}_{\text{rev}} \coloneqq \sum_{k=1}^d \ketbra{\epsilon_{d+1-k}}{\epsilon_k} & E \leq \epsilon_{\text{mean}} \,,\\
            \hat{\mathbb{I}} & E \geq \epsilon_{\text{mean}} \,.
        \end{cases}
    \end{align}
    We have that for any state this unitary extracts \emph{exactly} the energy-constrained minimum ergotropy and anti-ergotropy, i.e.,
    \begin{align}
        \forall\,\rho\in\sigma_E^{(\hat{H})},\quad
        &\Delta E^{(\hat{H}_{\text{as}})} (\rho, \hat{U}_{\text{rev}}^{(+,E)})
        = \mathcal{E}_{\text{min}}^{(\hat{H})}(E) \,,\\
        \forall\,\rho\in\sigma_E^{(\hat{H})},\quad
        &\Delta E^{(\hat{H}_{\text{as}})} (\rho,\hat{U}_{\text{rev}}^{(-,E)})
        = -\mathcal{A}_{\text{min}}^{(\hat{H})}(E)
    \end{align}
\end{theorem}
\begin{proof}
    We show that the given unitary $\hat{U}_{\text{rev}}^{(\pm,E)}$ extracts and charges an amount of energy equal to the energy-constrained minimum ergotropy and anti-ergotropy from every state $\rho$.
    Let $\hat{H}_{\text{as}} = \sum_{k=1}^d \epsilon_k \ketbra{\epsilon_k}{\epsilon_k}$ be an anti-symmetric Hamiltonian, and assume without loss of generality that the eigenvalues are already ordered, i.e., $\epsilon_{\text{min}} \equiv \epsilon_1 \leq \epsilon_2 \leq \dots \leq \epsilon_d \equiv \epsilon_{\text{max}}$ and for all $k$ we have $\epsilon_k + \epsilon_{d+1-k} = \epsilon_{\text{min}} + \epsilon_{\text{max}}$.
    We recall that for these Hamiltonians it follows that $\epsilon_{\text{mean}} = (\epsilon_{\text{min}} + \epsilon_{\text{max}})/2$ and (see Lemma~\ref{lemma:min-anti-erg-anti-h})
    \begin{align}
        \mathcal{E}_{\text{min}}^{(\hat{H}_{\text{as}})}(E)
        &= \begin{cases}
            0 & \text{ if }E\leq\epsilon_{\text{mean}} \,,\\
            2(E-\epsilon_{\text{mean}}) & \text{ if }E\geq\epsilon_{\text{mean}} \,,
        \end{cases} \\
        \mathcal{A}_{\text{min}}^{(\hat{H}_{\text{as}})}(E)
        &= \begin{cases}
            2(\epsilon_{\text{mean}}-E) & \text{ if }E\leq\epsilon_{\text{mean}} \,,\\
            0 & \text{ if }E\geq\epsilon_{\text{mean}} \,.
        \end{cases}
    \end{align}
    It is already clear that in the cases in which $\hat{U}_{\text{rev}}^{(\pm,E)}$ is equal to the identity, the energy variation is zero and matches the energy-constrained minimum ergotropy and anti-ergotropy.
    Let $\rho = \sum_{i,j} \rho_{ij} \ket{\epsilon_i} \bra{\epsilon_j}$ be any state expressed in the basis of the Hamiltonian.
    Its energy $E \equiv E(\rho)$ is
    \begin{align}
        E \equiv E(\rho)
        &= \trace\!\left[ \rho \hat{H}_{\text{as}} \right] \,,\\
        &= \sum_k \epsilon_k \rho_{kk} \,.
    \end{align}
    Now let $\tilde{\rho} = \hat{U}_{\text{rev}} \rho \hat{U}_{\text{rev}}^\dagger$ be the state with the inverted populations.
    Its energy $E(\tilde{\rho})$ is
    \begin{align}
        E(\tilde{\rho})
        &= \trace\!\left[ \hat{U}_{\text{rev}} \rho \hat{U}_{\text{rev}}^\dagger \hat{H}_{\text{as}} \right] \,,\\
        &= \sum_k \epsilon_{d+1-k} \rho_{kk} \,,\\
        &= \sum_k \left( 2 \epsilon_{\text{mean}} -\epsilon_{k} \right) \rho_{kk} \,,\\
        &= 2 \epsilon_{\text{mean}} - E \,,
    \end{align}
    where we exploited that the sum of the populations is one, $\sum_k \rho_{kk} = 1$.
    It is clear then that
    \begin{align}
        \Delta E^{(\hat{H}_{\text{as}})} (\rho,\hat{U}_{\text{rev}})
        &= E(\rho) - E(\tilde{\rho}) \,,\\
        &= 2 ( E(\rho) - \epsilon_{\text{mean}} ) \,,
    \end{align}
    which is exactly equal to the energy-constrained minimum ergotropy and minus the energy-constrained minimum anti-ergotropy in the desired energy ranges.
\end{proof}

\subsection{\label{subsec:diag}Structure of the optimal unitaries and diagonal states}

Thanks to Prop.~\ref{prop:minAreOrdered} we know that the minimum states for the ergotropy and anti-ergotropy are always passive and anti-passive states.
As a result, if you have that to extract or charge optimal energy \emph{from those states} you either apply the identity channel (no energy extractable or chargeable) $\mathcal{I}(\bullet) = \hat{\mathbb{I}} \bullet \hat{\mathbb{I}}$ or you invert the populations with the channel $\Lambda_{\text{rev}}(\bullet) = \hat{U}_{\text{rev}} \bullet \hat{U}_{\text{rev}}^\dagger$, where
\begin{align}\label{eq:rev-unitary}
    \hat{U}_{\text{rev}} \coloneqq \sum_{k=1}^d \ketbra{\epsilon_{d+1-k}}{\epsilon_k} \,,
\end{align}
and $\hat{H} = \sum_{k=1}^d \epsilon_k \ketbra{\epsilon_k}{\epsilon_k}$ is the Hamiltonian of the system.
This channel sends passive states into anti-passive states and vice versa, hence being optimal for the charging of the first and discharging of the latter.
As we already mentioned in the introduction of this section, in general, the energy you can extract from a state knowing only its mean energy is strictly lower than the energy-constrained minimum ergotropy  $\tilde{\mathcal{E}}^{(\hat{H})}(E) < \mathcal{E}^{(\hat{H})}_{\text{min}}(E)$ (and similarly for charging and anti-ergotropy).
This implies that while the channel $\Lambda_{\text{rev}}(\bullet)$ guarantees to extract (charge) at least $\mathcal{E}^{(\hat{H})}_{\text{min}}(E)$ ($\mathcal{A}^{(\hat{H})}_{\text{min}}(E)$) from all anti-passive states $\Delta_{E,\uparrow}^{(\hat{H})}$ (passive states $\Delta_{E,\downarrow}^{(\hat{H})}$), it does not extract (charge) in general this energy from all states $\rho\in\sigma_E^{(\hat{H})}$.
In fact, since this channel acts only on the ``diagonal energy" of the state, it does not obtain the desired result even for all states in $\Delta_E^{(\hat{H})}$.

It is reasonable to assume that if we restrict ourselves to a set $\mathcal{S} \subset \sigma_E^{(\hat{H})}$ small enough of the states, we will be able to extract or charge at least the energy-constrained minimum ergotropy or anti-ergotropy.
As it turns out, this is already possible by taking $\mathcal{S} \equiv \Delta_E^{(\hat{H})}$, i.e., all diagonal states.
But we just said that the channel $\Lambda_{\text{opt}}$ is \emph{not} optimal for all diagonal states (as we will see explicitly for the qutrit in Sec.~\ref{sec:qutrit}).
As it turns out, when restricting to diagonal states, one can achieve the desired result with a different quantum channel.
The following result is equivalent to the first part of Th.~4 of the main text.
\begin{theorem}[Part of Th.~4 of main text]\label{th:unk-extr-diag-states}
    Let $\hat{H}$ be a known finite-dimensional Hamiltonian, and let $\rho\in\Delta_E^{(\hat{H})}$ be a diagonal state of known mean energy $E$.
    Then, there exists a unitary quantum channel $\Lambda_{\max,\Delta}^{(\pm,E)}$ that guarantees to extract ($+$) and charge ($-$) at least the energy-constrained minimum ergotropy $\mathcal{E}_{\text{min}}^{(\hat{H})}$ ($+$) and anti-ergotropy ($-$) $\mathcal{A}_{\text{min}}^{(\hat{H})}$ from it, i.e.,
    \begin{align}
        \tilde{\mathcal{E}}_{\Delta}^{(\hat{H})}(E)
        \coloneqq \max_{\Lambda \in \mathcal{U}} \min_{\rho \in \Delta_E^{(\hat{H})}} \left[ \Delta E^{(\hat{H})} (\rho,\Lambda) \right]
        &= \min_{\rho \in \Delta_E^{(\hat{H})}} \max_{\Lambda \in \mathcal{U}} \left[ \Delta E^{(\hat{H})} (\rho,\Lambda) \right]
        \equiv \mathcal{E}_{\text{min}}^{(\hat{H})}(E) \,, \label{eq:ergprofo}\\
        \tilde{\mathcal{A}}_{\Delta}^{(\hat{H})}(E)
        \coloneqq \max_{\Lambda \in \mathcal{U}} \min_{\rho \in \Delta_E^{(\hat{H})}} \left[ - \Delta E^{(\hat{H})} (\rho,\Lambda) \right]
        &= \min_{\rho \in \Delta_E^{(\hat{H})}} \max_{\Lambda \in \mathcal{U}} \left[ - \Delta E^{(\hat{H})} (\rho,\Lambda) \right]
        \equiv \mathcal{A}_{\text{min}}^{(\hat{H})}(E) \,.
    \end{align}
\end{theorem}
\begin{proof}
We will prove the statement for $\tilde{\mathcal{E}}_{\Delta}^{(\hat{H})}(E)$, the proof for $\tilde{\mathcal{A}}_{\Delta}^{(\hat{H})}(E)$ follows similar steps.
It is sufficient to show that the $\min$ and the $\max$ in the right hand side of Eq.~\eqref{eq:ergprofo} commute.
Since $\mathcal{U}$ is not a convex set, we can not straightforwardly use the Sion minimax theorem \cite{sion1958minimax}.
We circumvent this issue by noticing that, for all $\rho \in \Delta_E^{(\hat{H})}$
\begin{align}
   \max_{\Lambda \in \mathcal{U}} \left[ \Delta E^{(\hat{H})} (\rho,\Lambda) \right] =  \max_{\Lambda' \in \mathcal{\mathcal{B}}} \left[ \Delta E^{(\hat{H})} (\rho,\Lambda') \right], \label{eq:permequi}
\end{align}
where $\mathcal{B}$ is the set of bistochastic maps, i.e., convex combinations of permutations of the energy levels.
To show Eq.~\eqref{eq:permequi} we first notice that $\Delta E^{(\hat{H})} (\rho,\Lambda) $ depends only on the diagonal part of $\Lambda(\rho)$.
Hence, for every $\Lambda$ we can construct an auxiliary map $\Lambda|_{\rm diag}$ that behaves as $\Lambda$ on the diagonal elements of $\rho \in \Delta_E^{\hat{H}}$ and, as a consequence, is such that $\Delta E^{(\hat{H})}(\rho, \Lambda) = \Delta E^{(\hat{H})}(\rho, \Lambda|_{\rm diag})$. This map is
\begin{equation}
 \Lambda|_{\rm diag}(\rho) \coloneqq \sum_{i,j=1}^d \braket{\epsilon_j|U|\epsilon_i}\braket{\epsilon_i|\rho|\epsilon_i} \braket{\epsilon_i|U^{\dag}|\epsilon_j} \ket{\epsilon_j} \bra{\epsilon_j} = 
 \sum_{i,j=1}^d P_{i,j} \braket{\epsilon_i|\rho|\epsilon_i}  \ket{\epsilon_j} \bra{\epsilon_j} ,
\end{equation}
where $P_{i,j} \coloneqq |\braket{\epsilon_i|U^{\dag}|\epsilon_j}|^2$.
Since $\sum_i P_{i,j} = \sum_j P_{i,j} =1$  we have $\Lambda|_{\rm diag} \in \mathcal{B}$. 
We have just shown that for every unitary we can construct a bistochastic map that achieves the same performance (and vice-versa). This proves Eq.~\eqref{eq:permequi}
and allows us to write
\begin{align}
    \min_{\rho \in \Delta_E^{(\hat{H})}} \max_{\Lambda \in \mathcal{U}} \left[ \Delta E^{(\hat{H})} (\rho,\Lambda) \right] =
    \min_{\rho \in \Delta_E^{(\hat{H})}} \max_{\Lambda' \in \mathcal{B}} \left[ \Delta E^{(\hat{H})} (\rho,\Lambda') \right] 
        = \max_{\Lambda' \in \mathcal{B}} \min_{\rho \in \Delta_E^{(\hat{H})}} \left[ \Delta E^{(\hat{H})} (\rho,\Lambda') \right],
\end{align}
where we used that $\mathcal{B}$ is a convex set and applied the minimax theorem.    
To conclude the theorem, it is sufficient to use again that the sets $\mathcal U$ and $\mathcal B$ behaves in the same way on $\Delta E^{(\mathcal{H})}$, so we can replace $\max_{\Lambda' \in \mathcal B}$ with $\max_{\Lambda \in \mathcal U} $.
\end{proof}

We have now shown that there exists a unitary quantum channel $\Lambda_{\max,\Delta}^{(\pm,E)}$ that guarantees the extraction and charging of at least the energy-constrained minimum ergotropy and anti-ergotropy from diagonal states. However, we previously claimed that this is not achieved by taking as unitary the one $\hat{U}_{\text{rev}}$ that reverses the populations.
So, what is the optimal unitary $\hat{U}_{\max,\Delta}^{(\pm,E)}$ for diagonal states?
It is in general not trivial to determine its structure, as we will see in the qutrit example  (Sec.~\ref{sec:qutrit}).
Nevertheless, we can give it a good characterization thanks to our knowledge of the states of energy-constrained minimum ergotropy and anti-ergotropy.
Taking as example the ergotropy, let $\tilde{\rho}(E)$ be the \emph{unique}\footnote{When the state is not unique, usually it means that the Hamiltonian is anti-symmetric and the problem simplifies significantly.} state that minimizes it for an energy value $E>\epsilon_{\text{mean}}$, i.e.,
\begin{align}
    \tilde{\rho}(E) = \arg \min_{\rho\in\sigma_E^{(\hat{H})}} \mathcal{E}^{(\hat{H})}(\rho) \,.
\end{align}
Thanks to Theorem~\ref{th:minErg} we know that this state will be in the form
\begin{align}
    \tilde{\rho}(E) = p \rho_{a}^\uparrow + (1-p) \rho_{b}^\uparrow \,,
\end{align}
where $1\leq a \leq b \leq d$, and the states $\rho_k^\uparrow$ are the basis (Eq.~\eqref{eq:basis-anti-passive}) of the simplex $\Delta_{\uparrow}^{(\hat{H})}$.
This state has at most three different eigenvalues (two if $a=1$).
The eigenvalue $\lambda_1=0$ has multiplicity $a-1$.
The eigenvalue $\lambda_2= \frac{p}{d+1-a}$ has multiplicity $b-a$.
Finally, the eigenvalue $\lambda_3 = \frac{p}{d+1-a} + \frac{1-p}{d+1-b}$ has multiplicity $d+1-b$.
It follows that in these three subspaces the state is proportional to the identity, and all the unitaries
\begin{align}
    \mathcal{V}(E) \ni \hat{V} \coloneqq \hat{U}_{\text{rev}} \left( \hat{U}_{1,a-1} \otimes \hat{U}_{a,b-1} \otimes \hat{U}_{b,d} \right) \,,
\end{align}
are optimal for extracting energy from this worst-case state, where $\hat{U}_{a,b}$ is a \emph{generic} local unitary acting on the subspace generated by $\{ \ket{\epsilon_a}, \dots , \ket{\epsilon_{b-1}} \}$.
One can easily check that this is indeed the case, since
\begin{align}
    \hat{V} \tilde{\rho}(E) \hat{V}^\dagger
    &= \hat{U}_{\text{rev}} \left( \hat{U}_{1,a-1} \otimes \hat{U}_{a,b-1} \otimes \hat{U}_{b,d} \right) \tilde{\rho}(E) \left( \hat{U}_{1,a-1}^\dagger \otimes \hat{U}_{a,b-1}^\dagger \otimes \hat{U}_{b,d}^\dagger \right) \hat{U}_{\text{rev}}^\dagger \,,\\
    &= \hat{U}_{\text{rev}} \tilde{\rho}(E) \hat{U}_{\text{rev}}^\dagger \,,
\end{align}
and, as we know, the reverse unitary $\hat{U}_{\text{rev}}$ is optimal for passive and anti-passive states.

While this argument does not provide explicitly the optimal unitary $\hat{U}_{\max,\Delta}^{(+,E)}$, it tells us that
\begin{align}\label{eq:opt-uni-diag-structure}
    \hat{U}_{\max,\Delta}^{(+,E)} \in \mathcal{V}(E)
    \quad\Rightarrow\quad
    \hat{U}_{\max,\Delta}^{(+,E)} = \hat{U}_{\text{rev}} \left( \hat{U}_{1,a-1}^* \otimes \hat{U}_{a,b-1}^* \otimes \hat{U}_{b,d}^* \right) \,,
\end{align}
where $\hat{U}_{1,a}^*$, $\hat{U}_{a,b-1}^*$, and $\hat{U}_{b,d}^*$ are three fixed unitary matrices (which may vary for different value of the mean energy $E$).
The latter is true because the optimal unitary $\hat{U}_{\max,\Delta}^{(+,E)}$ guarantees to extract at least the energy-constrained minimum ergotropy from all diagonal states, including the worst-case state, and the set $\mathcal{V}(E)$ was defined to be the set of all unitary matrices that extract all the energy from the worst-case state.
Hence, it must be $\hat{U}_{\max,\Delta}^{(+,E)} \in \mathcal{V}(E)$.

\subsection{\label{subsec:rand}Random unitaries}
In the previous section we saw that, by restricting to the study of diagonal states, we can safely extract at least the energy-constrained minimum ergotropy from every state, knowing simply its mean energy.
This is no longer true when considering the set of all states $\sigma_E^{(\hat{H})}$, hence, the unitary $\hat{U}_{\max,\Delta}^{(+,E)}$ that is optimal for diagonal states is no longer optimal in general if the state has coherences.
As you will see explicitly for the qutrit (Sec.~\ref{sec:qutrit}), this is indeed the case because if $\hat{U}_{\max,\Delta}^{(+,E)}$ extracts energy from a coherent part of $\rho$, then we can typically define another $\tilde{\rho}$, with the same mean energy, for which the unitary $\hat{U}_{\max,\Delta}^{(+,E)}$ increases the energy of the same coherent part.
The solution to this problem is to use random unitaries so that these positive and negative coherent contributions average to zero for all states, and we safely extract or charge energy into the diagonal part of the state.
\begin{definition}
   A quantum channel $\Lambda$ is a random unitary channel $\Lambda\in\mathcal{RU}$ if and only if it can be written as a convex sum of unitary channels, i.e.,
    \begin{align}
        \Lambda\in\mathcal{RU}
        \quad\Leftrightarrow\quad
        \Lambda(\bullet) = \sum_k p_k \hat{U}_k \bullet \hat{U}_k^\dagger \,,
    \end{align}
    where $\{ p_k \}_k $ is a probability distribution and $\{\hat{U}_k \}_k $ are unitary matrices $\hat{U}_k$.
\end{definition}
Contrary to the set of unitary matrices $\mathcal{U}$, the set of random unitary matrices $\mathcal{RU}$ is convex.
Thus, we can once again invoke the $\min-\max$ theorems to switch the minimum and the maximum in our definition of extractable (chargeable) energy and recover once again that it equals the energy-constrained minimum ergotropy (anti-ergotropy).
The following result is equivalent to the second part of Th.~4 of the main text.
\begin{theorem}[Part of Th.~4 of main text]\label{th:unk-extr-rand-uni}
    Let $\hat{H}$ be a known finite-dimensional Hamiltonian, and let $\rho\in\sigma_E^{(\hat{H})}$ be a state of known mean energy $E$.
    Then, there exists a random unitary quantum channel $\Lambda_{\max,\mathcal{RU}}^{(\pm,E)} \in \mathcal{RU}$ that guarantees the extraction and charging of at least the energy-constrained minimum ergotropy $\mathcal{E}_{\text{min}}^{(\hat{H})}$ and anti-ergotropy $\mathcal{A}_{\text{min}}^{(\hat{H})}$ from it, i.e.,
    \begin{align}
        \tilde{\mathcal{E}}_{\mathcal{RU}}^{(\hat{H})}(E)
        \coloneqq \max_{\Lambda \in \mathcal{RU}} \min_{\rho \in \sigma_E^{(\hat{H})}} \left[ \Delta E^{(\hat{H})} (\rho,\Lambda) \right]
        &= \min_{\rho \in \sigma_E^{(\hat{H})}} \max_{\Lambda \in \mathcal{RU}} \left[ \Delta E^{(\hat{H})} (\rho,\Lambda) \right]
        \equiv \mathcal{E}_{\text{min}}^{(\hat{H})}(E) \,,\\
        \tilde{\mathcal{A}}_{\mathcal{RU}}^{(\hat{H})}(E)
        \coloneqq \max_{\Lambda \in \mathcal{RU}} \min_{\rho \in \sigma_E^{(\hat{H})}} \left[ - \Delta E^{(\hat{H})} (\rho,\Lambda) \right]
        &= \min_{\rho \in \sigma_E^{(\hat{H})}} \max_{\Lambda \in \mathcal{RU}} \left[ - \Delta E^{(\hat{H})} (\rho,\Lambda) \right]
        \equiv \mathcal{A}_{\text{min}}^{(\hat{H})}(E) \,.
    \end{align}
\end{theorem}
\begin{proof}
    The minimax theorem, in one of its many forms~\cite{simons_minimax_1995} states that we can exchange the order of the $\max$ and the $\min$ provided that:
    \begin{itemize}
        \item The sets $\mathcal{RU}$ and $\sigma_E^{(\hat{H})}$ with respect to which we are doing the maximization and minimization are compact and convex.
        \item The function $\pm \Delta E^{(\hat{H})}(\rho,\Lambda)$ is quasi-concave with respect to the second argument, i.e., with respect to the quantum channel.
        \item The function $\pm \Delta E^{(\hat{H})}(\rho,\Lambda)$ is quasi-convex with respect to the first argument, i.e., with respect to the states.
    \end{itemize}
    Once we verify all of these hypotheses, the thesis holds.
    It is well known that the set $\mathcal{RU}$ of random unitaries is compact and convex.
    We recall that the same holds for the set $\sigma_E^{(\hat{H})}$ of all the states with mean energy $E$, since it is a linear subspace of the convex and compact space $\sigma(\mathcal{H})$.
    We are left with the task of showing that the function $\pm \Delta E^{(\hat{H})}(\rho,\Lambda)$ is quasi-convex with respect to the first argument and quasi-concave with respect to the second one.
    In fact, the function is linear with respect to both arguments.
    Let $\alpha, \beta \in \mathbb{R}$ be two numbers; we have
    \begin{align}
        \pm \Delta E^{(\hat{H})}(\alpha \rho_1 + \beta \rho_2,\Lambda)
        &= \trace\!\left[ \hat{H} \left( \alpha \rho_1 + \beta \rho_2 \right) \right] - \trace\!\left[ \hat{H} \Lambda \left( \alpha \rho_1 + \beta \rho_2 \right) \right] \,,\\
        &= \alpha \trace\!\left[ \hat{H} \rho_1 \right] + \beta \trace\!\left[ \hat{H} \rho_2 \right] - \trace\!\left[ \hat{H}\left( \alpha \Lambda (\rho_1) + \beta \Lambda (\rho_2) \right) \right] \,,\\
        &= \alpha \trace\!\left[ \hat{H} \rho_1 \right] + \beta \trace\!\left[ \hat{H} \rho_2 \right] - \alpha \trace\!\left[ \hat{H} \Lambda (\rho_1) \right] - \beta \trace\!\left[ \hat{H} \Lambda (\rho_2) \right] \,,\\
        &= \alpha \Delta E^{(\hat{H})}(\rho_1, \Lambda) + \beta \Delta E^{(\hat{H})} (\rho_2, \Lambda) \,,
    \end{align}
    where we have exploited the linearity of the trace operator and of quantum channels.
    We have thus shown that the target function is linear with respect to the first argument; by repeating the same kind of steps for the second one, one shows that it is also linear with respect to the second argument.
    It follows that all the hypotheses of the minimax theorem are fulfilled, thus we can exchange the $\min$ and the $\max$.
\end{proof}

\subsection{\label{subsec:lowerbound}Discussion \& a lower bound}

We did not find the optimal unitary in the general scenario of all states of known mean energy, but we have found three good candidates.
The first one is the unitary that reverses the populations:
\begin{align}
    \Lambda_{\text{rev}}(\bullet)
    = \hat{U}_{\text{rev}} \bullet \hat{U}_{\text{rev}}^\dagger \,,
    \qquad
    \hat{U}_{\text{rev}} \coloneqq \sum_{k=1}^d \ketbra{\epsilon_{d+1-k}}{\epsilon_k} \,,
\end{align}
where $\hat{H} = \sum_{k=1}^d \epsilon_k \ketbra{\epsilon_k}{\epsilon_k}$ is the Hamiltonian of the system with the eigenvalues ordered ($\epsilon_k \leq \epsilon_{k+1}$).
This unitary is good because it is independent of the mean energy and it is a permutation in the Hamiltonian basis; hence, you will not have a problem of inadvertently charge energy through the coherence of a state when it is not diagonal.
The only problem related to this choice is that, for an arbitrary Hamiltonian $\hat{H}$, this may not be very good for all diagonal states.

The second one is the unitary which is optimal for diagonal states, which we did not find in general but of which we provided insights in its structure:
\begin{align}\label{eq:diag-state-channel}
    \Lambda_{\max,\Delta}^{(\pm,E)}(\bullet)
    = \hat{U}_{\max,\Delta}^{(\pm,E)} \bullet \hat{U}_{\max,\Delta}^{(\pm,E)\dagger} \,,
    \qquad
    \hat{U}_{\max,\Delta}^{(\pm,E)} \coloneqq \hat{U}_{\text{rev}} \left( \hat{U}_{1,a-1}^* \otimes \hat{U}_{a,b-1}^* \otimes \hat{U}_{b,d}^* \right) \,,
\end{align}
where $a,b$ are indices determined by the value of the mean energy $E$, as well as the specific local unitaries $\hat{U}_{x,y}^*$ (which usually are not unique but have some extra degrees of freedom). 
This choice is good because it extracts (or charges) at least the minimum value of the ergotropy (or anti-ergotropy).
The problem of this choice is that the unitary $\hat{U}_{\max,\Delta}^{(\pm,E)}$ is not a permutation; hence, it can increase the energy of a state if it has coherences.

The remaining choice, no longer unitary, involves considering a random unitary channel, as discussed in Sec.~\ref{subsec:rand}.
While we did not discuss how to construct such a unitary channel, we want to present an intuitive picture of it (and the explicit construction will be provided for the qutrit in Sec.~\ref{sec:qutrit}).
The key point is that, in general, the quantum unitary channel $\Lambda_{\max,\Delta}^{(\pm,E)}(\bullet)$ which is optimal for diagonal states is not unique.
Many different possible choices $\{ \Lambda_{\max,\Delta}^{(\pm,E)}(\bullet,\Vec{\alpha}) \}_{\Vec{\alpha}}$ can be constructed such that their action on diagonal states is equivalent, but their action on non-diagonal states yields different results.
While we cannot construct a quantum unitary channel $\Lambda_{\max,\Delta}^{(\pm,E)}(\bullet, \Vec{\alpha}^*)$ such that for all non-diagonal states we will extract a positive amount of energy from the coherences, we can average over the possible choices,
\begin{align}
    \Lambda_{\max,\mathcal{RU}}^{(\pm,E)}(\bullet)
    \coloneqq \sum_{\Vec{\alpha}} p_{\Vec{\alpha}} \Lambda_{\max,\Delta}^{(\pm,E)}(\bullet, \Vec{\alpha}) \,,
\end{align}
so that for all states such contribution will be zero.

While this coherent contribution can indeed create problems, it is natural to guess that as $E$ gets closer to the maximum available energy, $\epsilon_{\text{max}}$, coherences will go to zero and the optimal unitary for diagonal states will work better and better.
This can be easily shown with a not tight lower bound.
\begin{lemma}
    Let $\rho\in\sigma_E^{(\hat{H})}$ be any state, and let $\Lambda_{\max,\Delta}^{(\pm,E)}$ be the unitary quantum channel that is optimal for diagonal states (Eq.~\eqref{eq:diag-state-channel}) for energy extraction and charging, respectively.
    We have
    \begin{align}
        \Delta E ( \rho, \Lambda_{\max,\Delta}^{(+,E)})
        &\geq \mathcal{E}_{\text{min}}^{(\hat{H})}(E) - \sqrt{2\ln2} \epsilon_{\text{max}} \sqrt{S(\omega_{\beta(E)})} \,,\\
        - \Delta E ( \rho, \Lambda_{\max,\Delta}^{(-,E)})
        &\geq \mathcal{A}_{\text{min}}^{(\hat{H})}(E) - \sqrt{2\ln2} \epsilon_{\text{max}} \sqrt{S(\omega_{\beta(E)})} \,,
    \end{align}
    where $S(\omega_{\beta(E)}) \coloneqq -\trace [\omega_{\beta(E)}\log\omega_{\beta(E)}]$ is the entropy of the Gibbs (or anti-Gibbs, depending on the value of $E$) state $\omega_{\beta(E)}$, having mean energy $E$.
\end{lemma}
As $E\rightarrow\epsilon_{\text{max}}$, we have that $\omega_{\beta(E)} \simeq \ketbra{\epsilon_{\text{max}}}{\epsilon_{\text{max}}}$ and, as a consequence, $S(\omega_{\beta(E)}) \simeq 0$.
This guarantees us in a quantitative way that as the energy increases, the optimal unitary channel presented extracts a positive and possibly great amount of energy.
Also, this is exactly what we expect, since as the energy of a state approaches the maximum possible energy the coherences must decrease, hence the unitary quantum channel which is optimal for diagonal states will become more and more suitable for all states.
\begin{proof}
    Exploiting the fact that the state $\rho\in\sigma_E^{(\hat{H})}$ and its dephased counterpart $\Delta(\rho)$ have the same mean energy, we can write
    \begin{align}
        \Delta E ( \rho, \Lambda_{\max,\Delta}^{(\pm,E)}
        &= \trace\!\left[\hat{H} \rho \right] - \trace\!\left[\hat{H} \Lambda_{\max,\Delta}^{(\pm,E)}(\rho) \right] \,,\\
        &= \overbrace{\left( \trace\!\left[\hat{H} \Delta(\rho) \right] - \trace\!\left[\hat{H} \Lambda_{\max,\Delta}^{(\pm,E)}(\Delta(\rho)) \right] \right)}^{\eqqcolon \Delta E_{\text{inc}}^\pm} - \overbrace{\left( \trace\!\left[\hat{H} \and
        \Lambda_{\max,\Delta}^{(\pm,E)}(\rho) \right] - \trace\!\left[\hat{H} \Lambda_{\max,\Delta}^{(\pm,E)}(\Delta(\rho)) \right] \right)}^{\eqqcolon \Delta E_{\text{coh}}^\pm} \,,
    \end{align}
    where we added and subtracted the energy of the diagonal state evolved with the same optimal unitary.
    In this way, we have divided the energy variation due to the action of the channel on the incoherent and coherent parts of $\rho$.
    By definition, since the unitary quantum channel used is optimal for diagonal states, we have
    \begin{align}
        \Delta E_{\text{inc}}^+
        &= \Delta E ( \Delta(\rho), \Lambda_{\max,\Delta}^{(+,E)})
        \geq \mathcal{E}_{\text{min}}^{(\hat{H})}(E) \,,\\
        \Delta E_{\text{inc}}^-
        &= \Delta E ( \Delta(\rho), \Lambda_{\max,\Delta}^{(-,E)})
        \leq -\mathcal{A}_{\text{min}}^{(\hat{H})}(E) \,.
    \end{align}
    Let us now look at the coherent contribution 
    \begin{align}
        \left| \Delta E_{\text{coh}}^\pm \right|
        &= \left| \trace\!\left[\hat{H} \hat{U}_{\max,\Delta}^{(\pm,E)} \rho \hat{U}_{\max,\Delta}^{(\pm,E) \dagger} \right] - \trace\!\left[\hat{H} \hat{U}_{\max,\Delta}^{(\pm,E)} \Delta(\rho) \hat{U}_{\max,\Delta}^{(\pm,E) \dagger} \right] \right| \,,\\
        &= \left| \trace\!\left[ \hat{U}_{\max,\Delta}^{(\pm,E) \dagger} \hat{H} \hat{U}_{\max,\Delta}^{(\pm,E)} \left( \rho - \Delta(\rho)\right) \right] \right| \,,\\
        &\leq \left|\left| \hat{U}_{\max,\Delta}^{(\pm,E) \dagger} \hat{H} \hat{U}_{\max,\Delta}^{(\pm,E)} \right|\right|_\infty \left|\left| \rho - \Delta(\rho) \right|\right|_1 \,,\\
        &= \epsilon_{\text{max}} \left|\left| \rho - \Delta(\rho) \right|\right|_1 \,,
    \end{align}
    where we exploited the cyclicity of the trace, the H\"older's inequality~\cite{stein2009real}, and the fact that by applying a unitary transformation to $\hat{H}$ we do not change its eigenvalues.
    The inequality we applied is far from optimal because, for this energetic contribution, we lost along the way all the information about the unitary used.
    Despite this limitation, we expect that the trace distance $\frac{1}{2}||\rho-\Delta(\rho)||_1$ tends to zero as the energy increases, and this can indeed be shown.
    We now aim to upper-bound this trace distance in terms of something that depends only on the energy of the state.
    In order to do so, we exploit the quantum Pinsker inequality~\cite{qpinskereasy},
    \begin{align}
        ||\rho-\Delta(\rho)||_1^2
        \leq 2\ln2 D(\rho||\Delta(\rho)) \,,
    \end{align}
    where $D(\rho||\Delta(\rho))$ is the quantum relative entropy~\cite{wilde2016} between the two states.
    Fortunately, the quantum relative entropy between a state and its dephased version simplifies significantly:
    \begin{align}
        D(\rho||\Delta(\rho))
        &= \trace\!\left[ \rho \log \rho \right] - \trace\!\left[ \rho \log \Delta(\rho) \right] \,,\\
        &= \trace\!\left[ \rho \log \rho \right] - \trace\!\left[ \Delta(\rho) \log \Delta(\rho) \right] \,,\\
        &= - S(\rho) + S(\Delta(\rho)) \equiv C(\rho) \,,
    \end{align}
    where $S(\bullet)$ is the entropy and $C(\bullet)$ is the \emph{relative entropy of coherence}~\cite{PhysRevLett.113.140401}.
    We have
    \begin{align}
        C(\rho) \leq \max_{\rho\in\sigma_E^{(\hat{H})}} C(\rho) \leq \max_{\rho\in\sigma_E^{(\hat{H})}} S(\Delta(\rho)) = \max_{\rho\in\Delta_E^{(\hat{H})}}S(\rho) = S(\omega_{\beta(E)}) \,,
    \end{align}
    where $\omega_{\beta(E)} = e^{-\beta(E)\hat{H}}/Z(\beta(E))$ is the Gibbs or anti-Gibbs state that has mean energy $E$.
    Note that, in the last step, we used the fact that the state of maximum of entropy with fixed mean energy $E$ is exactly the Gibbs or anti-Gibbs, depending on the value of $E$~\cite{PhysRev.106.620}.
    This inequality can in fact be saturated by taking the pure pseudo-Gibbs (or pseudo-anti-Gibbs) state, i.e., $\rho = \ketbra{\Psi}{\Psi}$ with $\ket{\Psi} = \sum_k \sqrt{e^{-\beta(E)\epsilon_k}/Z(\beta(E))} \ket{\epsilon_k}$.
    Thus, we have
    \begin{align}
        \left| \Delta E_{\text{coh}}^\pm \right| \leq \epsilon_{\text{max}} \sqrt{||\rho-\Delta(\rho)||_1^2} \leq \epsilon_{\text{max}} \sqrt{2\ln2 S(\omega_{\beta(E)})} \,,
    \end{align}
    
    By combining the two bounds for the incoherent and coherent contribution, we get the desired result.
    \begin{align}
        \Delta E ( \rho, \Lambda_{\max,\Delta}^{(+,E)})
        &= \Delta E_{\text{inc}}^+ - \Delta E_{\text{coh}}^+ \geq \mathcal{E}_{\text{min}}^{(\hat{H})}(E) - \epsilon_{\text{max}}\sqrt{2\ln2 S(\omega_{\beta(E)})} \,,
    \end{align}
    and
    \begin{align}
        \Delta E ( \rho, \Lambda_{\max,\Delta}^{(-,E)})
        &= \Delta E_{\text{inc}}^- - \Delta E_{\text{coh}}^- \leq -\mathcal{A}_{\text{min}}^{(\hat{H})}(E) + \epsilon_{\text{max}}\sqrt{2\ln2 S(\omega_{\beta(E)})} \,.
    \end{align}
\end{proof}
As we already mentioned this lower bound is not optimal, and the reason is that while bounding the coherent contribution to the energy we do not do any optimization with respect to the unitary that we use.
Nevertheless, it allows us to quantitatively say that as long as the mean energy increases (or decreases for the charging), the unitary evolution which is optimal for diagonal states becomes increasingly effective for coherent states.

\section{\label{sec:qutrit}Detailed calculations for the qutrit example}

We now want to work out all the calculations for a generic qutrit in order to compare the performances in energy extraction of the unitaries $\hat{U}_{\text{rev}}$ (Eq.~\eqref{eq:rev-unitary}), which is not in general optimal for all diagonal states, and $\hat{U}_{\max,\Delta}^{(\pm,E)}$ (Eq.~\eqref{eq:opt-uni-diag-structure}), which is optimal for all diagonal states but mixes populations and coherences, hence, it can be detrimental if the state has coherences.

Without loss of generality, let our Hamiltonian be $\hat{H} = \sum_{k=1}^3 \epsilon_k \ketbra{\epsilon_k}{\epsilon_k}$, where
\begin{align}
    \epsilon_1 = 0 \,,\qquad
    \epsilon_2 = (1+\delta)\epsilon \,,\qquad
    \epsilon_3 = 2\epsilon \,,
\end{align}
where $\epsilon\in(0,+\infty)$ and $\delta\in[-1,1]$, so that by construction $\epsilon_1 \leq \epsilon_2 \leq \epsilon_3$.

\subsection{\label{subsec:qutrit-min-erg}Energy-constrained minimum ergotropy of the qutrit}

The basis of the simplex of anti-passive states (see Sec.~\ref{subsec:min-state-charac}) is
\begin{align}
    \rho_1^\uparrow
    &= \frac{1}{3} \left( \ketbra{\epsilon_1}{\epsilon_1} + \ketbra{\epsilon_2}{\epsilon_2} + \ketbra{\epsilon_3}{\epsilon_3} \right) \,,\\
    \rho_2^\uparrow
    &= \frac{1}{2} \left( \ketbra{\epsilon_2}{\epsilon_2} + \ketbra{\epsilon_3}{\epsilon_3} \right) \,,\\
    \rho_3^\uparrow
    &= \ketbra{\epsilon_3}{\epsilon_3} \,.
\end{align}
Their mean energies and ergotropies are
\begin{align}
    \label{eq:qutrit-anti-pass-1}
    &E_1 \coloneqq E(\rho_1^\uparrow) = \epsilon \left(1 + \frac{\delta}{3}\right) = \epsilon_{\text{mean}} \,,
    &\mathcal{E}_1 \coloneqq \mathcal{E}^{(\hat{H})}(\rho_1^\uparrow) = 0 \,,\\
    \label{eq:qutrit-anti-pass-2}
    &E_2 \coloneqq E(\rho_2^\uparrow) = \epsilon\left(\frac{3}{2} + \frac{\delta}{2}\right) = \frac{3}{2}\epsilon_{\text{mean}} \,,
    &\mathcal{E}_2 \coloneqq \mathcal{E}^{(\hat{H})}(\rho_2^\uparrow) = \epsilon \,,\\
    \label{eq:qutrit-anti-pass-3}
    &E_3 \coloneqq E(\rho_3^\uparrow) = 2\epsilon \,,
    &\mathcal{E}_3 \coloneqq \mathcal{E}^{(\hat{H})}(\rho_3^\uparrow) = 2\epsilon \,.
\end{align}
We already know that the energy-constrained minimum ergotropy in the area $[\epsilon_1,\epsilon_{\text{mean}}]$ is zero due to the existence of passive states.
We want to find its value in the area $[\epsilon_{\text{mean}},\epsilon_3]$.
There are two possible scenarios.
\begin{enumerate}
    \item The energy-constrained minimum ergotropy is given by the states $(1-p) \rho_1^\uparrow + p \rho_3^\uparrow$ ($p\in[0,1]$) in the whole area $[\epsilon_{\text{mean}},\epsilon_3]$.
    \item The energy-constrained minimum ergotropy is given by the states $(1-p) \rho_1^\uparrow + p \rho_2^\uparrow$ in the area $[\epsilon_{\text{mean}},\frac{3}{2}\epsilon_{\text{mean}}]$ and by the states $(1-p) \rho_2^\uparrow + p \rho_3^\uparrow$ in the area $[\frac{3}{2}\epsilon_{\text{mean}},\epsilon_3]$.
\end{enumerate}
Also, if $\delta=0$ we return to the anti-symmetric scenario in which both cases return the same results.
Since we have only three energy levels, we can compare the two scenarios simply by comparing the ergotropies $\mathcal{E}_2$ of the state $\rho_2^\uparrow$ and $\Bar{\mathcal{E}}$ of the state $(1-\Bar{p}) \rho_1^\uparrow + \Bar{p} \rho_3^\uparrow$, with probability $\Bar{p}$ chosen such that its mean energy $\Bar{E}$ is equal to the one of $\rho_2^\uparrow$, $\Bar{E} = E_2$.
We have
\begin{align}
    &\mathcal{E}^{(\hat{H})}((1-\Bar{p})\rho_1^\uparrow + \Bar{p} \rho_3^\uparrow)
    \leq \mathcal{E}^{(\hat{H})}(\rho_2^\uparrow) \,,\\
    \Leftrightarrow\quad &\Bar{p} \cdot 2\epsilon
    \leq \epsilon \,,\\
    \Leftrightarrow\quad &\Bar{p} \leq \frac{1}{2} \,,
\end{align}
where we have exploited the linearity of the ergotropy with respect to anti-passive states.
We now know the correct scenario based on the probability of the state.
Our aim, though, is to find the energy-constrained minimum ergotropy with respect to the spectrum of the qutrit.
To do so, we need to write the probability $\Bar{p}$ in terms of the mean energy.
Exploiting the linearity of the mean energy, we have
\begin{align}
    \frac{3}{2} \epsilon_{\text{mean}}
    &= E_2 \,,\\
    &= E ((1-\Bar{p})\rho_1^\uparrow + \Bar{p} \rho_3^\uparrow) \,,\\
    &= (1-\Bar{p})E(\rho_1^\uparrow) + \Bar{p} E(\rho_3^\uparrow) \,,\\
    &= (1-\Bar{p}) \epsilon_{\text{mean}} + \Bar{p} \cdot 2\epsilon \,,\\
    &= \epsilon_{\text{mean}} + \Bar{p} (2\epsilon - \epsilon_{\text{mean}}) \,,
\end{align}
from which we get
\begin{align}
    \Bar{p} &= \frac{\frac{1}{2}\epsilon_{\text{mean}}}{2\epsilon - \epsilon_{\text{mean}}} \,,\\
    &= \frac{1}{2}\cdot\frac{3+\delta}{3-\delta} \,,
\end{align}
from which it is easy to see that $\Bar{p} \leq \frac{1}{2} \Leftrightarrow \delta \leq 0$.
Thus, we have that the correct scenario is the first ($1.$) iff $\delta \leq 0$, while it is the second ($2.$) iff $\delta > 0$, as summarised by Fig.~\ref{fig:min-erg-qutrit}.
\begin{figure}[t]
    \centering
    \includegraphics[width=0.8\linewidth]{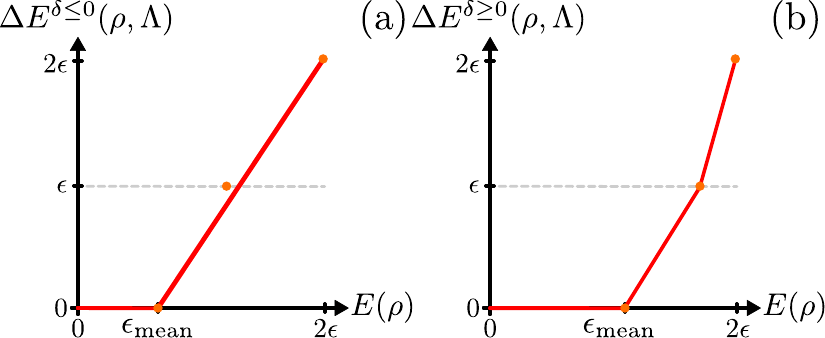}
    \caption{energy-constrained minimum ergotropy with respect to the mean energy $\mathcal{E}^{(\hat{H})}_{\text{min}}(E)$ (red line) for the qutrit when the intermediate energy level $\epsilon_2=\epsilon(1+\delta)$ is closer to the ground state $\epsilon_1=0$ than to the maximally excited state $\epsilon_3 = 2\epsilon$ (i.e., $\delta\leq0$, figure (a) (left)) and viceversa (i.e., $\delta\geq0$, figure (b) (right)).
    The orange dots represents the energies and ergotropies $(E_k,\mathcal{E}_k)$ for the three vertexes of the set of all anti-passive states (see Eqs.~\eqref{eq:qutrit-anti-pass-1},~\eqref{eq:qutrit-anti-pass-2}, and~\eqref{eq:qutrit-anti-pass-3}).
    } 
    \label{fig:min-erg-qutrit}
\end{figure}

We now want to evaluate explicitly these minimum ergotropies in terms of the parameter $\delta$ and the mean energy $E$.
In general, since the mean energy is linear with respect to all states and the ergotropy is linear with respect to passive and anti-passive states, we have that if the anti-passive state $\Bar{\rho}(p) = (1-p) \rho_a^\uparrow + p \rho_b^\uparrow$ (where $\rho_a^\uparrow, \rho_b^\uparrow$ are anti-passive) has mean energy $E$, the probability $p = p(E)$ can be written in terms of the mean energies $E_a, E_b$ of the two states as
\begin{align}
    p(E) = \frac{E-E_a}{E_b - E_a} \,,
\end{align}
and the ergotropy of $\Bar{\rho}(p)$ can be written in terms of the original ergotropies $\mathcal{E}_a, \mathcal{E}_b$ as
\begin{align}
    \mathcal{E}^{(\hat{H})}(\Bar{\rho})
    &= \mathcal{E}_a + p (\mathcal{E}_b - \mathcal{E}_a) \,,\\
    &= \mathcal{E}_a + \frac{\mathcal{E}_b - \mathcal{E}_a}{E_b - E_a} (E-E_a) \,.
\end{align}
It follows that, for the qutrit, the energy-constrained minimum ergotropy can be written as
\begin{align}
    \mathcal{E}_{\text{min}}^{\delta\leq0}(E)
    &= \begin{cases}
        0 & \text{if } E\in[0,\epsilon_{\text{mean}}] \,,\\
        \frac{2\epsilon}{2\epsilon-\epsilon_{\text{mean}}} \left( E - \epsilon_{\text{mean}} \right) & \text{if } E\in[\epsilon_{\text{mean}},2\epsilon] \,,
    \end{cases} \\
    \mathcal{E}_{\text{min}}^{\delta\geq0}(E)
    &= \begin{cases}
        0 & \text{if } E\in[0,\epsilon_{\text{mean}}] \,,\\
        \frac{2\epsilon}{\epsilon_{\text{mean}}} \left( E - \epsilon_{\text{mean}} \right) & \text{if } E\in[\epsilon_{\text{mean}},\frac{3}{2}\epsilon_{\text{mean}}] \,,\\
        \epsilon + \frac{\epsilon}{2\epsilon-\frac{3}{2}\epsilon_{\text{mean}}} \left( E - \frac{3}{2}\epsilon_{\text{mean}} \right) & \text{if } E\in[\frac{3}{2}\epsilon_{\text{mean}}, 2\epsilon] \,.
    \end{cases}
\end{align}

\subsection{\label{subsec:qutrit-rev}Performances of the reverse-unitary}
Let us now study the worst-case scenario performances of $\hat{U}_{\text{rev}}$, which for the qutrit can be written explicitly as
\begin{align}
    \hat{U}_{\text{rev}}
    &= \sum_{k=1}^3 \ketbra{\epsilon_{d+1-k}}{\epsilon_k} \,,\\
    &= \ketbra{\epsilon_3}{\epsilon_1} + \ketbra{\epsilon_1}{\epsilon_3} + \ketbra{\epsilon_2}{\epsilon_2} \,,
\end{align}
i.e., the unitary simply swaps the ground state $\ket{\epsilon_1}$ and the maximally excited state $\ket{\epsilon_3}$.
This unitary does not mix populations and coherences; hence, while studying energy variations, we can reduce ourselves to the study of diagonal states $\rho_\Delta$,
\begin{align}
    \rho_\Delta = p_1 \ketbra{\epsilon_1}{\epsilon_1} + p_2 \ketbra{\epsilon_2}{\epsilon_2} + p_3 \ketbra{\epsilon_3}{\epsilon_3} \,,
\end{align}
where, as usual, $p_1+p_2+p_3 = 1$ and $p_1,p_2,p_3\geq0$.
The energy extracted (or charged) from such states through the unitary $\hat{U}_{\text{rev}}$ is simply
\begin{align}
    \Delta E^{(\hat{H})} (\rho_\Delta, \Lambda_{\text{rev}})
    &= (p_3 - p_1) \epsilon_3 \,,\\
    &= 2\epsilon (p_3 - p_1) \,.
\end{align}
We want to find the minimum of such energy variation with respect to all possible populations, with the constraint of a given mean energy.
Let $E_\Delta$ be the mean energy of $\rho_\Delta$, we can write it in terms of the populations of the state as
\begin{align}
    E_\Delta
    &= E(\rho_\Delta) \,,\\
    &= p_1 \epsilon_1 + p_2 \epsilon_2 + p_3 \epsilon_3 \,,\\
    &= (1-p_1-p_3) \epsilon_2 + p_3 \epsilon_3 \,,\\
    &= \epsilon_2 - p_1 \epsilon_2 + p_3 (\epsilon_3 - \epsilon_2) \,.
\end{align}
We can now exploit this constraint to rewrite the energy variation $\Delta E$ between the initial and the final state in terms of the mean energy $E_\Delta$ and only one free parameter $p_3$.
\begin{align}
    \Delta E^{(\hat{H})} (\rho_\Delta, \Lambda_{\text{rev}})
    &= \frac{\epsilon_3}{\epsilon_2} ( p_3 \epsilon_2 - p_1 \epsilon_2 )  \,,\\
    &= \frac{\epsilon_3}{\epsilon_2} \left[ p_3 \epsilon_2 + E_\Delta - \epsilon_2 - p_3 (\epsilon_3 - \epsilon_2) \right] \,,\\
    &= \frac{\epsilon_3}{\epsilon_2} \left[ E_\Delta - \epsilon_2 + p_3 (2\epsilon_2 - \epsilon_3) \right] \,.
\end{align}
We know that $(2\epsilon_2 - \epsilon_3) = 2\epsilon \delta$, thus, when $\delta < 0$ ($\delta > 0$) we want to maximize (minimize) the probability $p_3$.

Let us start by considering the case $\delta < 0$.
When the mean energy is fixed, in order to maximize the probability $p_3$ of the maximally excited state we want to choose $p_2 = 0$, a choice that is possible for all values of mean energy\footnote{It might seem counterintuitive to set the intermediate population to zero, but we have to keep in mind that we are now looking to the worst possible state with respect to the unitary $\hat{U}_{\text{rev}}$, not to the state with the energy-constrained minimum ergotropy. In general, the diagonal states with $p_2=0$ have higher ergotropies than anti-passive states with the same mean energy, but, when $\delta<0$, you extract less energy from them through $\hat{U}_{\text{rev}}$.}.
Thus, we have that the worst-case state $\rho_\Delta^{\delta < 0}$ can be written as
\begin{align}
    \rho_\Delta^{\delta < 0} = (1-p) \ketbra{\epsilon_1}{\epsilon_1} + p \ketbra{\epsilon_3}{\epsilon_3} \,,
\end{align}
and has mean energy $E_\Delta = p \epsilon_3 = 2\epsilon p$ and, through $\hat{U}_{\text{rev}}$, you extract an amount of energy equal to $(2p-1)\epsilon_3$.
Thus, the minimum extractable energy that you will extract from a state having mean energy $E$ through the unitary $\hat{U}_{\text{rev}}$, when $\delta \leq 0$, is
\begin{align}
    \Delta E^{\delta \leq 0}_{\text{min}} (E , \Lambda_{\text{rev}})
    &= 2 E - \epsilon_3 \,,\\
    &= 2 (E - \epsilon) \,.
\end{align}
We see that, when $\delta<0$, this will be smaller than the energy-constrained minimum ergotropy, since they are both straight lines passing through the point $(E,\mathcal{E}) = (2\epsilon,2\epsilon)$, but, while the energy-constrained minimum ergotropy intercept the $E$-axis in $(\epsilon_{\text{mean}},0)$, this minimum energy intercept the $E$-axis in $(\epsilon,0)$, and
\begin{align}
    \epsilon \stackrel{\delta<0}{>} \epsilon_{\text{mean}} = \epsilon \left( 1 + \frac{\delta}{3} \right) \,.
\end{align}

Let us now consider the case $\delta > 0$.
In order to minimize the energy variation $\Delta E$, we now need to minimize $p_3$.
The best possible scenario is then to set $p_3=0$.
This is indeed possible for some mean energy values $E>\epsilon_{\text{mean}}$.
Let us consider the state
\begin{align}
    \rho_{\Delta,1}^{\delta\geq0} = (1-p) \ketbra{\epsilon_1}{\epsilon_1} + p \ketbra{\epsilon_2}{\epsilon_2} \,.
\end{align}
This state has mean energy $p \epsilon_2$, and, when $\delta>0$, $\epsilon_2 = \epsilon(1+\delta) > \epsilon(1+\delta/3) = \epsilon_{\text{mean}}$.
It follows that for the mean energy values $E\in[\epsilon_{\text{mean}},\epsilon_2]$ you cannot safely extract energy through the unitary $\hat{U}_{\text{rev}}$, since the minimum extractable energy is
\begin{align}
    \Delta E^{\delta \geq 0}_{\text{min}} (E\in[\epsilon_{\text{mean}},\epsilon_2] , \Lambda_{\text{rev}})
    &= (p-1) \epsilon_3 \,,\\
    &= \left( \frac{E}{\epsilon_2} - 1 \right) \epsilon_3 \,,\\
    &= \frac{\epsilon_3}{\epsilon_2} (E - \epsilon_2) \leq 0 \,.
\end{align}
When $E>\epsilon_2$, though, we must have $p_3 > 0$.
In this case, in order to minimize the probability of $p_3$ we keep $p_1=0$, so that the mean energy constraint is satisfied by the smallest possible value of $p_3$.
Thus, the minimum state is
\begin{align}
    \rho_{\Delta,2}^{\delta\geq0} = (1-p) \ketbra{\epsilon_2}{\epsilon_2} + p \ketbra{\epsilon_3}{\epsilon_3} \,.
\end{align}
with mean energy $E = \epsilon_2 + p (\epsilon_3 - \epsilon_2)$, and the energy $\Delta E$ that you will extract from it has value
\begin{align}
    \Delta E^{\delta \geq 0}_{\text{min}} (E\in[\epsilon_2,\epsilon_3] , \Lambda_{\text{rev}})
    &= p \epsilon_3 \,,\\
    &= \frac{\epsilon_3}{\epsilon_3 - \epsilon_2} ( E-\epsilon_2 ) \,.
\end{align}
Again, since $\epsilon_2 > \epsilon_{\text{mean}}$, we find that the amount of energy we can safely extract with $\hat{U}_{\text{rev}}$ is non-zero for higher values of the mean energy with respect to the mean energy at which the ergotropy becomes positive.

To sum up, assuming that below the threshold at which the reverse unitary can actually charge the system we do not perform any operation, we can write the minimum extractable energy obtained by reversing the populations as
\begin{align}
    \Delta E^{\delta \leq 0}_{\text{min, rev}} (E)
    &= \begin{cases}
        0 & \text{if }E\in[0,\epsilon] \,,\\
        2E - \epsilon_3 & \text{if }E\in[\epsilon,\epsilon_3] \,,
    \end{cases} \\
    \Delta E^{\delta \geq 0}_{\text{min, rev}} (E)
    &= \begin{cases}
        0 & \text{if }E\in[0,\epsilon_2] \,,\\
        \frac{\epsilon_3}{\epsilon_3 - \epsilon_2} ( E-\epsilon_2 ) & \text{if }E\in[\epsilon_2,\epsilon_3] \,.
    \end{cases}
\end{align}
Note that, even though they are written with different notations, when $E\geq\frac{3}{2}\epsilon_{\text{mean}}$ we have that $\Delta E^{\delta \geq 0}_{\text{min, rev}} (E) = \mathcal{E}_{\text{min}}^{(\hat{H})}(E)$, i.e., the reverse unitary becomes optimal for high mean energy values.
These results are summarised in Fig.~\ref{fig:min-rev-qutrit}.
\begin{figure}[t]
    \centering
    \includegraphics[width=0.8\linewidth]{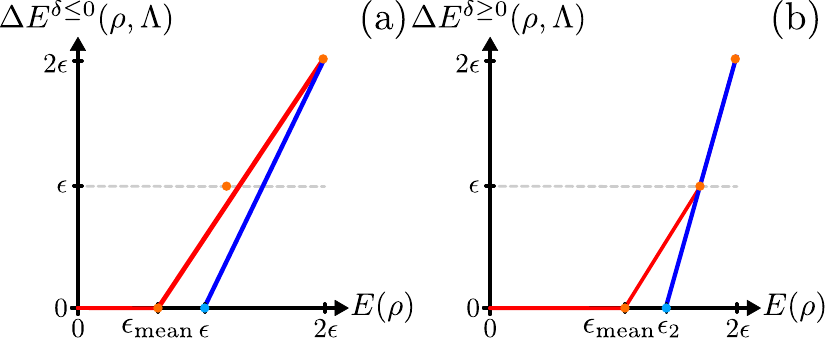}
    \caption{
        Minimum extractable energy $\Delta E_{\text{min, rev}}(E)$ through the unitary $\hat{U}_{\text{rev}}$ for the qutrit (blue line) in the two scenario $\delta\leq0$ (left figure, (a)) and $\delta\geq0$ (right figure, (b)).
        To avoid overlapping in the $E(\rho)$-axis, the figure of merit is displayed only when positive. 
        Red line represents the energy-constrained minimum ergotropy (for figure (b), partially overlapped with the red line) and orange dots the energy and ergotropy of the three vertexes of the set of all anti-passive states, as in Fig.~\ref{fig:min-erg-qutrit}.
    } 
    \label{fig:min-rev-qutrit}
\end{figure}

\subsection{\label{subsec:qutrit-opt}Performances of the diagonal optimal unitary}

We now want to find the explicit form of the optimal unitary $\hat{U}_{\max,\Delta}^{(+,E)}$ that, according to Theorem~\ref{th:unk-extr-diag-states}, should guarantee us to extract at least the energy-constrained minimum ergotropy from diagonal states.
We will now start with the scenario in which $\delta\geq0$.

Let us start by considering a mean energy $E\in[\epsilon_{\text{mean}},\frac{3}{2}\epsilon_{\text{mean}}]$.
For these mean energies, the anti-passive state which have energy-constrained minimum ergotropy, can be written as
\begin{align}\label{eq:qutrit-w-anti-passive}
    \rho_{\text{min}}^\uparrow(p)
    &= (1-p) \rho_1^\uparrow + p \rho_2^\uparrow \,,\\
    &= \left[ \frac{1}{3} - \frac{p}{3} \right] \ketbra{\epsilon_1}{\epsilon_1}
    + \left[ \frac{1}{3} + \frac{p}{6} \right] \ketbra{\epsilon_2}{\epsilon_2}
    + \left[ \frac{1}{3} + \frac{p}{6} \right] \ketbra{\epsilon_3}{\epsilon_3} \,,
\end{align}
where the value of $p\in[0,1]$ sets the mean energy $E = (1-p) \epsilon_{\text{mean}} + p \frac{3}{2} \epsilon_{\text{mean}}$.
Its ergotropy $\mathcal{E}^{(\hat{H})}(\rho_{\text{min}}^\uparrow) = \mathcal{E}_{\text{min}} (E(p))$ can be written explicitly in terms of the probability $p$ as
\begin{align}
    \mathcal{E}^{(\hat{H})}(\rho_{\text{min}}^\uparrow)
    &= \Delta E^{(\hat{H})} (\rho_{\text{min}}^\uparrow, \Lambda_{\text{rev}}) \,,\\
    &= \left( p_3 - p_1 \right) \epsilon_3 \,,\\
    &= p \epsilon \,,
\end{align}
where as usual $p_k$ is the population of the $k$-th energy level.
The most generic diagonal state $\rho_\Delta$ having the same mean energy as $\rho_{\text{min}}^\uparrow$ can be written as
\begin{align}
    \rho_\Delta(p)
    &= \lambda_1 \ketbra{\epsilon_1}{\epsilon_1} + \lambda_2 \ketbra{\epsilon_2}{\epsilon_2} + \lambda_3 \ketbra{\epsilon_3}{\epsilon_3} \,,\\
    &= \left[ \frac{1}{3} - \frac{p}{3} - (1-s)\Delta \right] \ketbra{\epsilon_1}{\epsilon_1}
    + \left[ \frac{1}{3} + \frac{p}{6} + \Delta \right] \ketbra{\epsilon_2}{\epsilon_2}
    + \left[ \frac{1}{3} + \frac{p}{6} - s \Delta \right] \ketbra{\epsilon_3}{\epsilon_3} \,,
\end{align}
where $s \coloneqq \frac{\epsilon_2}{\epsilon_3}$ so that the mean energy of the state $\rho_\Delta(p)$ is the same as the one of the state $\rho_{\text{min}}^\uparrow(p)$,
\begin{align}
    E ( \rho_\Delta(p) )
    &= E (\rho_{\text{min}}^\uparrow(p)) - (1-s) \Delta \epsilon_1 + \Delta \epsilon_2 - s \Delta \epsilon_3 \,,\\
    &= E (\rho_{\text{min}}^\uparrow(p)) \,,
\end{align}
and $\Delta$ is a number that can be either positive (if we want to increase the population of the central energy level) or negative (if we want to decrease it), constrained only by the necessity that all the populations $\lambda_k$ must be greater than or equal to zero.
As we have seen in the last section, the reverse unitary is not in general optimal for these diagonal states.
By construction, the optimal unitary $\hat{U}_{\max,\Delta}^{(+,E)}$ extracts an amount of energy at least equal to the energy-constrained minimum ergotropy from each diagonal state, as proven in Theorem~\ref{th:unk-extr-diag-states}.
It follows that such unitary will extract exactly the ergotropy from the states $\rho_{\text{min}}^\uparrow(p)$.
Hence, we can use these states to bound the possible structure of $\hat{U}_{\max,\Delta}^{(+,E)}$.
The most general unitary that extracts the ergotropy from the state $\rho_{\text{min}}^\uparrow(p)$ is an arbitrary unitary $\hat{U}_{23}$ acting only in the subspace generated by $\{ \ket{\epsilon_2},\ket{\epsilon_3} \}$ followed by the reverse unitary $\hat{U}_{\text{rev}}$.
Thus, it can be written as
\begin{align}
    \hat{U}_{\max,\Delta}^{(+,E)}
    &= \hat{U}_{\text{rev}} \overbrace{\left( \ketbra{\epsilon_1}{\epsilon_1} + \ketbra{\psi}{\epsilon_2} + \ketbra{\psi_\perp}{\epsilon_3} \right)}^{\eqqcolon \hat{U}_{23}} \,,\\
\end{align}
where $\ket{\psi}, \ket{\psi_\perp}$ are, in their most general structure,
\begin{align}
    \label{eq:psi-qutrit}
    \ket{\psi}
    &= e^{i\theta} \left[ \sqrt{1-q} \ket{\epsilon_2} + e^{i\phi} \sqrt{q} \ket{\epsilon_3} \right] \,,\\
    \label{eq:psi-perp-qutrit}
    \ket{\psi_\perp}
    &= e^{i\alpha} \left[ \sqrt{q} \ket{\epsilon_2} - e^{i\phi} \sqrt{1-q} \ket{\epsilon_3} \right] \,,
\end{align}
where $q\in[0,1]$ and $\theta,\phi,\alpha\in\mathbb{R}$.
The energy extracted from a generic diagonal state with the optimal unitary is
\begin{align}
    \Delta E^{(\hat{H})}(\rho_\Delta, \Lambda_{\max,\Delta}^{(+,E)})
    &= E(\rho_\Delta) - E\left(\hat{U}_{\max,\Delta}^{(+,E)} \rho_\Delta \hat{U}_{\max,\Delta}^{(+,E) \dagger} \right) \,,\\
    &= E(\rho_\Delta) - E\left( \hat{U}_{\text{rev}} \tilde{\rho}_\Delta \hat{U}_{\text{rev}}^\dagger \right) \,,\\
    &= \lambda_2 \epsilon_2 + \lambda_3 \epsilon_3 - \left( \tilde{\lambda}_2 \epsilon_2 + \tilde{\lambda}_1 \epsilon_3 \right) \,,\\
    &= \epsilon_3 \left( \lambda_3 - \tilde{\lambda}_1 \right) + \epsilon_2 \left( \lambda_2 - \tilde{\lambda}_2 \right) \,,
\end{align}
where $\tilde{\lambda}_k \coloneqq \braket{\epsilon_k|\tilde{\rho}_\Delta|\epsilon_k}$ are the populations of the state $\tilde{\rho}_\Delta \coloneqq \hat{U}_{23} \rho_\Delta \hat{U}_{23}^\dagger$.
We want to compute these populations and then optimise the free parameters of $\hat{U}_{23}$ so that the energy we extract is at least the energy-constrained minimum ergotropy for all diagonal states.
We have
\begin{align}
    \tilde{\rho}_\Delta
    &= \hat{U}_{23} \rho_\Delta \hat{U}_{23}^\dagger \,,\\
    &= \lambda_1 \ketbra{\epsilon_1}{\epsilon_1}
    + \lambda_2 \ketbra{\psi}{\psi}
    + \lambda_3 \ketbra{\psi_\perp}{\psi_\perp} \,,
\end{align}
from which we get
\begin{align}
    \tilde{\lambda}_1
    &= \braket{\epsilon_1| \left[ \lambda_1 \ketbra{\epsilon_1}{\epsilon_1}
    + \lambda_2 \ketbra{\psi}{\psi}
    + \lambda_3 \ketbra{\psi_\perp}{\psi_\perp} \right] |\epsilon_1} \,,\\
    &= \lambda_1 \,,
\end{align}
and
\begin{align}
    \tilde{\lambda}_2
    &= \braket{\epsilon_2| \left[ \lambda_1 \ketbra{\epsilon_1}{\epsilon_1}
    + \lambda_2 \ketbra{\psi}{\psi}
    + \lambda_3 \ketbra{\psi_\perp}{\psi_\perp} \right] |\epsilon_2} \,,\\
    &= \lambda_2 |\braket{\epsilon_2|\psi}|^2 + \lambda_3 |\braket{\epsilon_2|\psi_\perp}|^2 \,,\\
    &= \lambda_2 (1-q) + \lambda_3 q \,.
\end{align}
By substituting these expressions in the mean energy variations and writing the populations explicitly, we get
\begin{align}
    \Delta E^{(\hat{H})}(\rho_\Delta, \Lambda_{\max,\Delta}^{(+,E)})
    &= \epsilon_3 \left( \lambda_3 - \lambda_1 \right) + \epsilon_2 q \left( \lambda_2 - \lambda_3 \right) \,,\\
    &= \epsilon_3 \left( \frac{1}{3} + \frac{p}{6} - s \Delta - \left( \frac{1}{3} - \frac{p}{3} - (1-s) \Delta \right) \right) + \epsilon_2 q \left( \frac{1}{3} + \frac{p}{6} + \Delta - \left( \frac{1}{3} + \frac{p}{6} - s \Delta \right) \right) \,,\\
    &= \mathcal{E}_{\text{min}}^{(\hat{H})}(E(p)) + \Delta \left[ \epsilon_2 (1+s) q - \epsilon_3 (2s-1) \right] \,.
\end{align}
In general, since $s = \frac{\epsilon_2}{\epsilon_3}>\frac{1}{2}$ (for $\delta>0$), depending on the sign of $\Delta$ of the diagonal state in exam, we have that the extra contribution can be either positive or negative.
The only option is to choose $q$ exactly such that the extra term in the parenthesis cancel out, i.e.,
\begin{align}
    q \coloneqq \frac{2s-1}{s(s+1)} \,,
\end{align}
from which we get
\begin{align}
    \Delta E^{(\hat{H})}\left( \rho_\Delta, \left.\Lambda_{\max,\Delta}^{(+,E)}\right|_{q=q(E)} \right) = \mathcal{E}_{\text{min}}^{(\hat{H})} \left( E(\rho_\Delta) \right) \,.
\end{align}

The next step is to consider a general state with coherences and see how those affects the energy extraction performances with this protocol.
Let $\rho = \sum_{i,j=1}^3 \rho_{ij} \ketbra{\epsilon_i}{\epsilon_j}$ be any state (with mean energy $E\in[\epsilon_{\text{mean}},\frac{3}{2}\epsilon_{\text{mean}}]$).
We have
\begin{align}
    \Delta E^{(\hat{H})} (\rho, \Lambda_{\max,\Delta}^{(+,E)})
    &= E \left( \rho \right) - E \left( \hat{U}_{\max,\Delta}^{(+,E)} \rho \hat{U}_{\max,\Delta}^{(+,E) \dagger} \right) \,,\\
    &= \overbrace{E\left( \rho \right)
    - E\left( \hat{U}_{\max,\Delta}^{(+,E)} \Delta(\rho) \hat{U}_{\max,\Delta}^{(+,E) \dagger} \right)}^{ = \mathcal{E}_{\text{min}}^{(\hat{H})} (E(\rho)) }
    + \overbrace{E\left( \hat{U}_{\max,\Delta}^{(+,E)} \Delta(\rho) \hat{U}_{\max,\Delta}^{(+,E) \dagger} \right)
    - E\left( \hat{U}_{\max,\Delta}^{(+,E)} \rho \hat{U}_{\max,\Delta}^{(+,E) \dagger} \right)}^{\eqqcolon E_c(\rho,\hat{U}_{\text{opt}}) } \,,
\end{align}
where $\Delta(\rho)$ is the diagonal version of the state $\rho$.
We have
\begin{align}
    E_c(\rho, \Lambda_{\max,\Delta}^{(+,E)})
    &= \trace\! \left[ \hat{H} \hat{U}_{\max,\Delta}^{(+,E)} \left( \sum_{i \neq j} \rho_{ij} \ket{\epsilon_i}\bra{\epsilon_j} \right) \hat{U}_{\max,\Delta}^{(+,E) \dagger} \right] \,,\\
    &= 2 \sum_{i > j} \Re{ \rho_{ij} \overbrace{\trace\! \left[ \hat{H} \hat{U}_{\max,\Delta}^{(+,E)} \left( \ket{\epsilon_i}\bra{\epsilon_j} \right) \hat{U}_{\max,\Delta}^{(+,E) \dagger} \right]}^{\eqqcolon B_{ij}} } \,.
\end{align}
We have
\begin{align}
    B_{21} &= \trace\! \left[ \hat{H} \hat{U}_{\max,\Delta}^{(+,E)} \left( \ket{\epsilon_2}\bra{\epsilon_1} \right) \hat{U}_{\max,\Delta}^{(+,E) \dagger} \right] \,,\\
    &= \trace\! \left[ \hat{U}_{\text{rev}}^\dagger \hat{H} \hat{U}_{\text{rev}} \ket{\psi}\bra{\epsilon_1} \right] \,,\\
    &= \trace\! \left[ \hat{H}_{\text{rev}} \ket{\psi}\bra{\epsilon_1} \right] \,,\\
    &= 0 \,,\\
    B_{31} &= \trace\! \left[ \hat{H} \hat{U}_{\max,\Delta}^{(+,E)} \left( \ket{\epsilon_3}\bra{\epsilon_1} \right) \hat{U}_{\max,\Delta}^{(+,E) \dagger} \right] \,,\\
    &= \trace\! \left[ \hat{U}_{\text{rev}}^\dagger \hat{H} \hat{U}_{\text{rev}} \ket{\psi_\perp}\bra{\epsilon_1} \right] \,,\\
    &= \trace\! \left[ \hat{H}_{\text{rev}} \ket{\psi_\perp}\bra{\epsilon_1} \right] \,,\\
    &= 0 \,,\\
    B_{32} &= \trace\! \left[ \hat{H} \hat{U}_{\max,\Delta}^{(+,E)} \left( \ket{\epsilon_3}\bra{\epsilon_2} \right) \hat{U}_{\max,\Delta}^{(+,E) \dagger} \right] \,,\\
    &= \trace\! \left[ \hat{U}_{\text{rev}}^\dagger \hat{H} \hat{U}_{\text{rev}} \ket{\psi_\perp}\bra{\psi} \right] \,,\\
    &= \trace\! \left[ \hat{H}_{\text{rev}} \ket{\psi_\perp}\bra{\psi} \right] \,,\\
    &= e^{i(\alpha-\theta)} \epsilon_2 \sqrt{q(1-q)} \,,
\end{align}
where we have exploited the cyclicity of the trace operator and $\hat{H}_{\text{rev}} \coloneqq \sum_{k=1}^3 \epsilon_{d+1-k} \ketbra{\epsilon_k}{\epsilon_k}$.
It follows that
\begin{align}
    E_c(\rho, \Lambda_{\max,\Delta}^{(+,E)})
    &= 2 \epsilon_2 \sqrt{q(1-q)} \Re{ \rho_{23} e^{i(\alpha-\theta)} } \,,\\
    &\geq - 2 \epsilon_2 \sqrt{q(1-q)} \sqrt{\lambda_2(\rho) \lambda_3(\rho)} \,,\\
    &\geq - 2 \epsilon_2 \sqrt{q(1-q)} \cdot \overbrace{\max_{\rho\in\sigma_E^{(\hat{H})}} \sqrt{\lambda_2(\rho) \lambda_3(\rho)}}^{\eqqcolon f(E) } \,,
\end{align}
where $\lambda_k(\rho) = \rho_{kk}$ are the populations, and we exploited that for off-diagonal elements of a density matrix we have $|\rho_{ij}| \leq \sqrt{\rho_{ii}\rho_{jj}}$.
Note that you can always saturate the lower bound by taking the feasible choice $\rho_{23} = \sqrt{\lambda_{2}\lambda_{3}} e^{-i(\alpha-\theta + \pi)}$.
The function $f(E)$ can be evaluated analytically, and it yields
\begin{align}
    f(E) = \begin{cases}
        \frac{E}{2\sqrt{\epsilon_2\epsilon_3}} & \text{if } E\in[\epsilon_{\text{mean}},\frac{\epsilon_2\epsilon_3}{\frac32\epsilon_{\text{mean}}}] \,,\\
        \frac{\sqrt{(E-\epsilon_2)(\epsilon_3-E)}}{\epsilon_3-\epsilon_2} & \text{if } E\in[\frac{\epsilon_2\epsilon_3}{\frac32\epsilon_{\text{mean}}},\frac{3}{2}\epsilon_{\text{mean}}] \,.
    \end{cases}
\end{align}
After all these calculations, we are finally ready to write down the minimum energy you will extract using the optimal unitary for diagonal states in the energy range $E\in[\epsilon_{\text{mean}},\frac{3}{2}\epsilon_{\text{mean}}]$:
\begin{align}
    \min_{\rho\in\sigma_E^{(\hat{H})}}
    \Delta E^{(\hat{H})} (\rho, \Lambda_{\max,\Delta}^{(+,E)})
    &= \mathcal{E}_{\text{min}}^{(\hat{H})}(E)
        - 2 \epsilon_2 \sqrt{q(1-q)} \cdot \begin{cases}
        \frac{E}{2\sqrt{\epsilon_2\epsilon_3}}
        & \text{if } E\in[\epsilon_{\text{mean}},\frac{\epsilon_2\epsilon_3}{\frac32\epsilon_{\text{mean}}}] \,,\\
        \frac{\sqrt{(E-\epsilon_2)(\epsilon_3-E)}}{\epsilon_3-\epsilon_2} & \text{if } E\in[\frac{\epsilon_2\epsilon_3}{\frac32\epsilon_{\text{mean}}},\frac{3}{2}\epsilon_{\text{mean}}] \,,
    \end{cases}
\end{align}
We should now repeat all the steps for the energy range $E\in[\frac{3}{2}\epsilon_{\text{mean}},\epsilon_3]$.
But we already know the optimal solution in this area from the previous section, i.e., $\hat{U}_{\text{rev}}$ itself.
Thus, we have that the optimal unitary that guarantees us to extract exactly the energy-constrained minimum ergotropy from all diagonal states can be written as
\begin{align}
    \label{eq:qutrit-opt-uni}
    \hat{U}_{\max,\Delta}^{(+,E)}
    &= \begin{cases}
        \hat{\mathbb{I}} & \text{if } E\in[0,\epsilon_{\text{mean}}] \,,\\
        \hat{U}_{\text{rev}} \hat{U}_{23}(\Bar{q}) & \text{if } E\in[\epsilon_{\text{mean}},\frac{3}{2}\epsilon_{\text{mean}}] \,, \\
        \hat{U}_{\text{rev}} & \text{if } E \in [\frac{3}{2}\epsilon_{\text{mean}}, \epsilon_3] \,,
    \end{cases}
\end{align}
where
\begin{align}
    \hat{U}_{23}(q)
    &\coloneqq \ketbra{\epsilon_1}{\epsilon_1} + \ketbra{\psi(q)}{\epsilon_2} + \ketbra{\psi_\perp(q)}{\epsilon_3} \,,\\
    \ket{\psi(q)}
    &= e^{i\theta} \left[ \sqrt{1-q} \ket{\epsilon_2} + e^{i\phi} \sqrt{q} \ket{\epsilon_3} \right] \,,\\
    \ket{\psi_\perp(q)}
    &= e^{i\alpha} \left[ \sqrt{q} \ket{\epsilon_2} - e^{i\phi} \sqrt{1-q} \ket{\epsilon_3} \right] \,,\\
    \Bar{q}
    &= \frac{2s-1}{s(s+1)} \,,\\
    s
    &\coloneqq \frac{\epsilon_2}{\epsilon_3} = \frac{1}{2} \left( 1 + \delta \right) \,.
\end{align}
This unitary guarantees to extract from \emph{all} diagonal states at least the energy-constrained minimum ergotropy (exactly, for $E\leq\frac{3}{2}\epsilon_{\text{mean}}$), $\Delta E^{(\hat{H})}(\rho_\Delta\in\sigma_E^{(\hat{H})}, \Lambda_{\max,\Delta}^{(+,E)}) = \mathcal{E}_{\text{min}}^{(\hat{H})}(E)$, and the minimum energy that it extracts from \emph{any} state is
\begin{align}
    \nonumber
    \Delta E_{\text{min}}^{\delta \geq0} (E, \Lambda_{\max,\Delta}^{(+,E)})
    &= \min_{\rho\in\sigma_E^{(\hat{H})}}
    \Delta E^{(\hat{H})} (\rho, \Lambda_{\max,\Delta}^{(+,E)}) \,,\\
    \label{eq:qutrit-min-diag-opt}
    &\geq \mathcal{E}_{\text{min}}^{(\hat{H})}(E)
        - 2 \epsilon_2 \sqrt{q(1-q)} \cdot \begin{cases}
        0 & \text{if } E\in[0,\epsilon_{\text{mean}}] \,,\\
        \frac{E}{2\sqrt{\epsilon_2\epsilon_3}}
        & \text{if } E\in[\epsilon_{\text{mean}},\frac{\epsilon_2\epsilon_3}{\frac32\epsilon_{\text{mean}}}] \,,\\
        \frac{\sqrt{(E-\epsilon_2)(\epsilon_3-E)}}{\epsilon_3-\epsilon_2} & \text{if } E\in[\frac{\epsilon_2\epsilon_3}{\frac32\epsilon_{\text{mean}}},\frac{3}{2}\epsilon_{\text{mean}}] \,,\\
        0 & E \in [\frac{3}{2}\epsilon_{\text{mean}}, \epsilon_3] \,.
    \end{cases}
\end{align}
Note that this extractable energy is not continuous in $E = \epsilon_{\text{mean}}$ and $E = \frac{3}{2} \epsilon_{\text{mean}}$ due to the abrupt change in the unitary.
In Fig.~\ref{fig:min-opt-qutrit} we can observe this minimum extractable energy and compare it with the other figures of merit found for the qutrit.
\begin{figure}[t]
    \centering
    \includegraphics[width=0.4\linewidth]{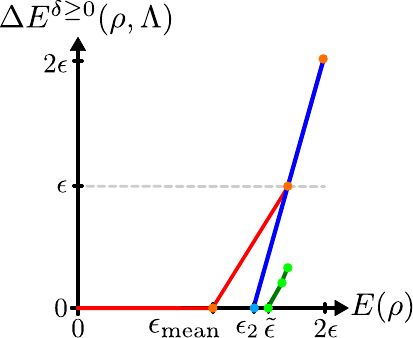}
    \caption{
        Comparison of the energy-constrained minimum ergotropy (red line), minimum extractable energy through the unitary $\hat{U}_{\text{rev}}$ that reverses the populations (blue line, displayed only when positive) and the minimum extractable energy through the unitary $\hat{U}_{\max,\Delta}^{(+,E)}$ that is optimal for diagonal states for a three-level system (green line, displayed only when positive in the mean energy range $E \in [ \epsilon_{\text{mean}} , \frac{3}{2} \epsilon_{\text{mean}}]$).
        The energy levels are $\epsilon_1=0$, $\epsilon_2=\epsilon(1+\delta)$ with $\delta\geq0$, and $\epsilon_3=2\epsilon$.
        As in Fig.~\ref{fig:min-rev-qutrit} (b), orange dots represents the vertexes of the simplex of anti-passive states and the light-blue dot represents the point $(\epsilon_2,0)$ at which the minimum extractable energy through the unitary $\hat{U}_{\text{rev}}$ becomes positive for all states.
        Similarly, the first light-green point $(\tilde{\epsilon},0)$, with $\epsilon_2 < \tilde{\epsilon} < \frac{3}{2} \epsilon_{\text{mean}}$ for $\delta>0$, represents the mean energy threshold at which the minimum extractable energy through the unitary $\hat{U}_{\max,\Delta}^{(+,E)}$ becomes positive for all states; the second light-green point is at the x-coordinate ($E= \frac{\epsilon_2\epsilon_3}{\frac{3}{2}\epsilon_{\text{mean}}}$, Eq.~\eqref{eq:qutrit-min-diag-opt}) at which the minimum changes its functional dependence with respect to the mean energy $E$, and the latter light-green point is at the x-coordinate $E = \frac{3}{2} \epsilon_{\text{mean}}$.
        }
    \label{fig:min-opt-qutrit}
\end{figure}

We will now quickly repeat all these steps for the scenario in which $\delta\leq0.$
As seen in the previous sections, in the whole mean energy range $E\in[\epsilon_{\text{mean}},\epsilon_3]$, the states having energy-constrained minimum ergotropy are a linear superposition of the completely mixed state and of the maximally excited state.
It follows that all diagonal states can be efficiently written as
\begin{align}
    \rho_\Delta(p)
    &= \lambda_1 \ketbra{\epsilon_1}{\epsilon_1} + \lambda_2 \ketbra{\epsilon_2}{\epsilon_2} + \lambda_3 \ketbra{\epsilon_3}{\epsilon_3} \,,\\
    &= \left[ \frac{1}{3} - \frac{p}{3} - (1-s)\Delta \right] \ketbra{\epsilon_1}{\epsilon_1}
    + \left[ \frac{1}{3} - \frac{p}{3} + \Delta \right] \ketbra{\epsilon_2}{\epsilon_2}
    + \left[ \frac{1}{3} + \frac{2p}{3} - s \Delta \right] \ketbra{\epsilon_3}{\epsilon_3} \,,
\end{align}
where again $s = \epsilon_2 / \epsilon_3$ so that the mean energy of $\rho_\Delta(p)$ depends only on $p$, $E(\rho_\Delta(p)) \equiv E(p) = \epsilon_{\text{mean}} + p (\epsilon_3 - \epsilon_{\text{mean}})$.
The energy-constrained minimum ergotropy of such a state when $E\geq\epsilon_{\text{mean}}$ is then
\begin{align}
    \mathcal{E}_{\text{min}}^{\delta\leq0}(E(p))
    &= \frac{\epsilon_3}{\epsilon_3 - \epsilon_{\text{mean}}} (E - \epsilon_{\text{mean}}) \,,\\
    &= p \epsilon_3 \,.
\end{align}
The worst-ergotropy states are now degenerate in the first and and second energy levels; the optimal unitary $\hat{U}_{\max,\Delta}^{(+,E)}$ that guarantees to extract at least the energy-constrained minimum ergotropy will be in the form
\begin{align}
    \hat{U}_{\max,\Delta}^{(+,E)}
    = \hat{U}_{\text{rev}} \overbrace{\left( \ketbra{\psi}{\epsilon_1} + \ketbra{\psi_\perp}{\epsilon_2} + \ketbra{\epsilon_3}{\epsilon_3} \right)}^{\eqqcolon \hat{U}_{12}} \,,
\end{align}
where, $\ket{\psi}$ and $\ket{\psi_\perp}$ will be in the form of Eqs.~\eqref{eq:psi-qutrit},~\eqref{eq:psi-perp-qutrit}.
We can again find the optimal value $\Bar{q}$ that defines $\hat{U}_{\max,\Delta}^{(+,E)}$ by working out the mean energy variation between the initial and the final state.
We have
\begin{align}
    \Delta E^{(\hat{H})}(\rho_\Delta, \Lambda_{\max,\Delta}^{(+,E)})
    &= E(\rho_\Delta) - E\left(\hat{U}_{\max,\Delta}^{(+,E)} \rho_\Delta \hat{U}_{\max,\Delta}^{(+,E) \dagger} \right) \,,\\
    &= E(\rho_\Delta) - E\left( \hat{U}_{\text{rev}} \tilde{\rho}_\Delta \hat{U}_{\text{rev}}^\dagger \right) \,,\\
    &= \lambda_2 \epsilon_2 + \lambda_3 \epsilon_3 - \left( \tilde{\lambda}_2 \epsilon_2 + \tilde{\lambda}_1 \epsilon_3 \right) \,,\\
    &= \epsilon_3 \left( \lambda_3 - \tilde{\lambda}_1 \right) + \epsilon_2 \left( \lambda_2 - \tilde{\lambda}_2 \right) \,,
\end{align}
where $\tilde{\lambda}_k \coloneqq \braket{\epsilon_k|\tilde{\rho}_\Delta|\epsilon_k}$ are the populations of the state $\tilde{\rho}_\Delta \coloneqq \hat{U}_{12} \rho_\Delta \hat{U}_{12}^\dagger$.
Let us compute those populations.
\begin{align}\tilde{\lambda}_1
    &= \braket{\epsilon_1| \left[ \lambda_1 \ketbra{\psi}{\psi}
    + \lambda_2 \ketbra{\psi_\perp}{\psi_\perp}
    + \lambda_3 \ketbra{\epsilon_3}{\epsilon_3} \right] |\epsilon_1} \,,\\
    &= \lambda_1 |\braket{\epsilon_1|\psi}|^2 + \lambda_2 |\braket{\epsilon_1|\psi_\perp}|^2 \,,\\
    &= \lambda_1 (1-q) + \lambda_2 q \,,\\
    \tilde{\lambda}_2
    &= \braket{\epsilon_2| \left[ \lambda_1 \ketbra{\psi}{\psi}
    + \lambda_2 \ketbra{\psi_\perp}{\psi_\perp}
    + \lambda_3 \ketbra{\epsilon_3}{\epsilon_3} \right] |\epsilon_2} \,,\\
    &= \lambda_1 |\braket{\epsilon_2|\psi}|^2 + \lambda_2 |\braket{\epsilon_2|\psi_\perp}|^2 \,,\\
    &= \lambda_1 q + \lambda_2 (1-q) \,;
\end{align}
from which we get
\begin{align}
    \Delta E^{(\hat{H})}(\rho_\Delta, \Lambda_{\max,\Delta}^{(+,E)})
    &= \epsilon_3 \left( \lambda_3 - \lambda_1 (1-q) - \lambda_2 q \right) + \epsilon_2 \left( \lambda_2 - \lambda_1 q - \lambda_2 (1-q) \right) \,,\\
    &= \epsilon_3 \left[ ( \lambda_3 - \lambda_1) + q ( 1 - s ) ( \lambda_1 - \lambda_2 ) \right] \,,\\
    &= \epsilon_3 \left[ p + (1-2s) \Delta - q ( 1 - s ) (2-s) \Delta \right] \,,\\
    &= \mathcal{E}_{\text{min}}(E(p)) + \epsilon_3 \Delta \left[ (1 - 2s) - q (1-s) (2-s) \right] \,.
\end{align}
We see that we can guarantee that $\Delta E^{(\hat{H})}(\rho_\Delta(p),\Lambda_{\max,\Delta}^{(+,E)}) = \mathcal{E}_{\text{min}}(E(p))$ for all diagonal states by choosing $q = \Bar{q}$,
\begin{align}
    \Bar{q} = \frac{1-2s}{(1-s)(2-s)} \,.
\end{align}
Now that we have characterized the optimal unitary, we want to evaluate its worst-case performances for arbitrary states (having coherences).
By redoing the same steps as in the scenario $\delta\geq0$, we have
\begin{align}
    \Delta E^{(\hat{H})} (\rho, \Lambda_{\max,\Delta}^{(+,E)})
    &= E \left( \rho \right) - E \left( \hat{U}_{\max,\Delta}^{(+,E)} \rho \hat{U}_{\max,\Delta}^{(+,E) \dagger} \right) \,,\\
    &= \overbrace{E\left( \rho \right)
    - E\left( \hat{U}_{\max,\Delta}^{(+,E)} \Delta(\rho) \hat{U}_{\max,\Delta}^{(+,E) \dagger} \right)}^{ = \mathcal{E}_{\text{min}}^{(\hat{H})} (E(\rho)) }
    + \overbrace{E\left( \hat{U}_{\max,\Delta}^{(+,E)} \Delta(\rho) \hat{U}_{\max,\Delta}^{(+,E) \dagger} \right)
    - E\left( \hat{U}_{\max,\Delta}^{(+,E)} \rho \hat{U}_{\max,\Delta}^{(+,E) \dagger} \right)}^{\eqqcolon E_c(\rho,\hat{U}_{\text{opt}}) } \,,
\end{align}
where $\Delta(\rho)$ is the diagonal version of the state $\rho$.
We have
\begin{align}
    E_c(\rho, \Lambda_{\max,\Delta}^{(+,E)})
    &= \trace\! \left[ \hat{H} \hat{U}_{\max,\Delta}^{(+,E)} \left( \sum_{i \neq j} \rho_{ij} \ket{\epsilon_i}\bra{\epsilon_j} \right) \hat{U}_{\max,\Delta}^{(+,E) \dagger} \right] \,,\\
    &= 2 \sum_{i > j} \Re{ \rho_{ij} \overbrace{\trace\! \left[ \hat{H} \hat{U}_{\max,\Delta}^{(+,E)} \left( \ket{\epsilon_i}\bra{\epsilon_j} \right) \hat{U}_{\max,\Delta}^{(+,E) \dagger} \right]}^{\eqqcolon B_{ij}} } \,,
\end{align}
and
\begin{align}
    B_{21} &= \trace\! \left[ \hat{H} \hat{U}_{\max,\Delta}^{(+,E)} \left( \ket{\epsilon_2}\bra{\epsilon_1} \right) \hat{U}_{\max,\Delta}^{(+,E) \dagger} \right] \,,\\
    &= \trace\! \left[ \hat{U}_{\text{rev}}^\dagger \hat{H} \hat{U}_{\text{rev}} \ket{\psi_\perp}\bra{\psi} \right] \,,\\
    &= \trace\! \left[ \hat{H}_{\text{rev}} \ket{\psi_\perp}\bra{\psi} \right] \,,\\
    &= \epsilon_3 e^{i(\alpha-\theta)} \sqrt{q(1-q)} (1-s) \,,\\
    B_{31} &=  0 \,,\\
    B_{32} &= 0 \,,
\end{align}
We now want to find the minimum of such coherent contribution,
\begin{align}
    E_c(\rho, \Lambda_{\max,\Delta}^{(+,E)})
    &= 2 \epsilon_3 \sqrt{q(1-q)} (1-s) \Re{ \rho_{12} e^{i(\alpha-\theta)} } \,,\\
    &\geq - 2 \epsilon_3 \sqrt{q(1-q)} (1-s) \sqrt{\lambda_1(\rho) \lambda_2(\rho)} \,,\\
    &\geq - 2 \epsilon_3 \sqrt{q(1-q)} (1-s) \cdot \overbrace{\max_{\rho\in\sigma_E^{(\hat{H})}} \sqrt{\lambda_1(\rho) \lambda_2(\rho)}}^{\eqqcolon f(E) } \,;
\end{align}
and again we can compute $f(E)$ explicitly, which yields the simpler (with respect to the previous case) expression
\begin{align}
    f(E) = \frac{\epsilon_3 - E}{2 \sqrt{\epsilon_3 ( \epsilon_3 - \epsilon_2 )}} \,.
\end{align}
We can now compute the minimum extractable energy through the optimal unitary,
\begin{align}
    \min_{\rho\in\sigma_E^{(\hat{H})}}
    \Delta E^{(\hat{H})} (\rho, 
    \Lambda_{\max,\Delta}^{(+,E)})
    &= \mathcal{E}_{\text{min}}^{(\hat{H})}(E) - \epsilon_3 (1-s) \sqrt{q(1-q)} \frac{\epsilon_3 - E}{\sqrt{\epsilon_3 (\epsilon_3 - \epsilon_2)}} \,,
\end{align}
where, we recall, it is assumed that $E \geq \epsilon_{\text{mean}}$.
\begin{figure}[t]
    \centering
    \includegraphics[width=0.4\linewidth]{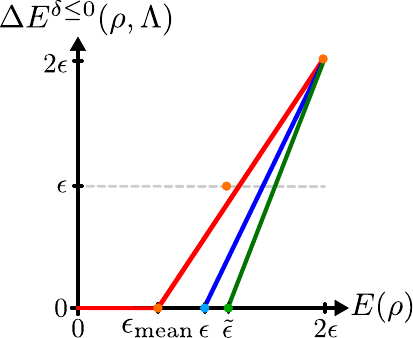}
    \caption{
        Comparison of the energy-constrained minimum ergotropy (red line), minimum extractable energy through the unitary $\hat{U}_{\text{rev}}$ that reverses the populations (blue line, displayed only when positive) and the minimum extractable energy through the unitary $\hat{U}_{\max,\Delta}^{(+,E)}$ that is optimal for diagonal states for a three-level system (green line, displayed only when positive).
        The energy levels are $\epsilon_1=0$, $\epsilon_2=\epsilon(1+\delta)$ with $\delta\leq0$, and $\epsilon_3=2\epsilon$.
        As in Fig.~\ref{fig:min-rev-qutrit} (a), orange dots represents the vertexes of the simplex of anti-passive states and the light-blue dot represents the point $(\epsilon,0)$ at which the minimum extractable energy through the unitary $\hat{U}_{\text{rev}}$ becomes positive for all states.
        Similarly, the light-green point $(\tilde{\epsilon},0)$, with $\epsilon < \tilde{\epsilon}$, represents the mean energy threshold at which the minimum extractable energy through the unitary $\hat{U}_{\max,\Delta}^{(+,E)}$ becomes positive for all states.}
    \label{fig:min-opt-qutrit-delta-leq-zero}
\end{figure}

\subsection{\label{subsec:qutrit-rand-uni}Optimal random unitary operations}
As we have seen in Sec.~\ref{subsec:rand}, through the use of random unitary channels we can again achieve the optimal performances, i.e.,
\begin{align}
    \tilde{\mathcal{E}}_{\mathcal{RU}}^{(\hat{H})}(E)
        \coloneqq \max_{\Lambda \in \mathcal{RU}} \min_{\rho \in \sigma_E^{(\hat{H})}} \left[ \Delta E^{(\hat{H})} (\rho,\Lambda) \right]
        = \min_{\rho \in \sigma_E^{(\hat{H})}} \max_{\Lambda \in \mathcal{RU}} \left[ \Delta E^{(\hat{H})} (\rho,\Lambda) \right]
        \equiv \mathcal{E}_{\text{min}}^{(\hat{H})}(E) \,.
\end{align}
In this final section, we want to verify this result for the qutrit explicitly and find the random unitary channel required to achieve these performances.

Let us start again to the scenario in which $\delta\geq0$.
We have seen that the optimal unitary for diagonal states is $\hat{U}_{\max,\Delta}^{(+,E)}$ as defined in Eq.~\eqref{eq:qutrit-opt-uni}.
This unitary already guarantees extracting at least the energy-constrained minimum ergotropy from all states in the energy ranges $E\in[0,\epsilon_{\text{mean}}]$ ($\hat{U}_{\max,\Delta}^{(+,E)} = \hat{\mathbb{I}}$) and $E\in[\frac{3}{2}\epsilon_{\text{mean}},\epsilon_3]$ ($\hat{U}_{\max,\Delta}^{(+,E)} = \hat{U}_{\text{rev}}$, as seen in Sec.~\ref{subsec:qutrit-rev}).
In the energy range $E\in[\epsilon_{\text{mean}},\frac{3}{2}\epsilon_{\text{mean}}]$ ($\hat{U}_{\max,\Delta}^{(+,E)} = \hat{U}_{\text{rev}} \hat{U}_{23}(\Bar{q})$) this is no longer the case, as seen in the previous section.
Despite that, the unitary $\hat{U}_{23}(\Bar{q})$ still has some free parameters $\alpha,\theta$ (so that $\hat{U}_{\max,\Delta}^{(+,E)} \equiv \hat{U}_{\max,\Delta}^{(+,E)}(\alpha,\theta)$) which do not affect the energy variation if the state is diagonal but do affect the energy variation if the state has coherences.
In particular, we have seen that in such energy range:
\begin{align}
    \Delta E^{(\hat{H})} (\rho, \Lambda_{\max,\Delta}^{(+,E)}(\alpha,\theta))
    &= \mathcal{E}^{(\hat{H})}_{\text{min}}(E(\rho)) + E_c(\rho,\Lambda_{\max,\Delta}^{(+,E)}(\alpha,\theta)) \,,\\
    &= \mathcal{E}^{(\hat{H})}_{\text{min}}(E(\rho)) + 2\epsilon_2 \sqrt{q(1-q)} \Re{\rho_{23}e^{i(\alpha-\theta)}} \,.
\end{align}
It is clear that the coherent energy contribution $E_c$ can be detrimental to energy extraction if the phases of $\rho_{23}$ are such that $\Re{\rho_{23}e^{i(\alpha-\theta)}} < 0$.
This situation can happen for any value of $\alpha,\theta$ so that there are no optimal parameters if we have access only to a single unitary.

If instead we have access to random unitary channels, we can take the same unitary with different phases so that the energy contribution due to coherences is always zero.
Specifically, let us consider the random unitary channel $\Lambda_{\max,\mathcal{RU}}^{(+,E)}$ defined as
\begin{align}
    \Lambda_{\max,\mathcal{RU}}^{(+,E)}(\rho)
    \coloneqq \frac12 \hat{U}_{\max,\Delta}^{(+,E)}(\alpha,\theta) \rho \hat{U}_{\max,\Delta}^{(+,E) \dagger}(\alpha,\theta)
    + \frac12 \hat{U}_{\max,\Delta}^{(+,E)}(\alpha+\pi,\theta) \rho \hat{U}_{\max,\Delta}^{(+,E) \dagger}(\alpha+\pi,\theta) \,,
\end{align}
where $\alpha$ and $\theta$ are arbitrary.
This channel is a combination of the optimal unitary for the qutrit with \emph{opposite} global phases.
The result is that the \emph{average} energy contribution due to the coherences will be zero for all states,
\begin{align}
    \Delta E^{(\hat{H})} (\rho,\Lambda_{\max,\mathcal{RU}}^{(+,E)})
    &= \frac{1}{2} \left( \mathcal{E}^{(\hat{H})}_{\text{min}}(E(\rho)) + 2\epsilon_2 \sqrt{q(1-q)} \Re{\rho_{23}e^{i(\alpha-\theta)}} \right)\\
    &+ \frac{1}{2} \left( \mathcal{E}^{(\hat{H})}_{\text{min}}(E(\rho)) + 2\epsilon_2 \sqrt{q(1-q)} \Re{\rho_{23}e^{i(\alpha-\theta)} e^{i\pi}} \right) \,\\
    &= \mathcal{E}^{(\hat{H})}_{\text{min}}(E(\rho)) \,,
\end{align}
where we have exploited that $\Re{z e^{i\pi}} = - \Re{z}$ for all complex numbers $z$.
Thus we have constructed a random unitary channel that extracts at least the energy-constrained minimum ergotropy from all states (and exactly that, if $E\leq\frac{3}{2}\epsilon_{\text{mean}}$).

The same steps can be repeated if $\delta\leq0$, thus building random unitary channels which extract \emph{exactly} the energy-constrained minimum ergotropy from every state.

\renewcommand{\theenumiv}{S\arabic{enumiv}}
\makeatletter
\renewcommand\@biblabel[1]{[S#1]}
\makeatother

\bibliography{bibliography}
\end{document}
